# Supplementary material for: ViLPAct: A Benchmark for Compositional Generalization on Multimodal Human Activities
Source: arXiv:2210.05556 source file (2023-03-09)
Supplement: Supplementary file 1 [file 08_appendix.tex]

\section{Dataset Creation \& Details}
\label{sec:dataset}
\subsection{Activity Extraction}
\label{alg:cap}
% With Algorithm \ref{act_algo},
\subsubsection{Overview}
We find that each video in \charades may contain multiple sequences of activities, consisting of related actions in temporal order, representing an event done by a person in the video. To collect the labelled temporal actions in a video, each action label inside is grouped to be a set of temporal action labels. Each temporal action label will be a triplet of action class, action start time and end time.
We first filter out 223 videos that don't have action set labels and 6622 videos that don't contain action sequences longer than 3. 
After filtering we get about 3003 videos, each of which consists of some action sequences that contain more than 3 actions. \\
However, from the observation, most of these remaining videos contain actions which represents activities with multiple intents. In order to preserve the core action sequence with a clear intent in the video which can be used to plan future actions, we need to design a greedy algorithm that explores an action sequence by expanding the most promising action in a limited action label set.
% Then we randomly selected one action sequence as an action sequence of this video. These examples contain 2371 non-repetitive action sequences, covering 148 of the 157 action classes.

\\
% We found that in \charades, a video may contain more than one activity, whereas we are more concerned with a single activity with a clear intent to do reasoning about future actions. Therefore, we design an activity (action sequence) extraction algorithm to organize the temporal activity chains from the action set of the \charades video. 
% This algorithm uses a greedy search that explores an action sequence by expanding the most promising action in a limited set. It uses text similarity, temporal relevance, and topic matching between two actions to find the most possible next action in the candidate set. The details are shown below.
\subsubsection{Algorithm Definitions}

\begin{algorithm}
\small
\SetAlgoNoLine  %去掉之前的竖线
\caption{Activity Extractor}
%\begin{algorithmic}
  \label{act_algo}  
  \KwIn{$Actions = \{a_1,a_2,\ldots ,a_n\}$, each action  $a_i = \left < cls^{a_i}, t_s^{a_i}, t_e^{a_i}\right >$ , where $cls^{a_i}$ is the action class, $t_s^{a_i}$ and  $t_e^{a_i}$is the start time and end time of action $a_i$. Relevance threshold }
  \KwOut{$Activities = \{A_1, A_2, \dots ,A_n\}$, where each activity represents an action sequence}
  Remaining actions set $R_a$ = $Actions$\\
  \While{R_a \neq $\emptyset$}
  {
        Sort $R_a$ in ascending order by start time $t_s$\\
        pre action $a = R_a[0]$\\
        Activity $A = \{a\}$\\
        $Search = True$\\
        \While{Search}{
            candidates $C_a = \{a_j \in R_a | t_s^{a_j} \ge t_s^{a}\}$\\
            \For{$a_j \in C_a$} 
            {
            Calculate relevance score = $s_{a_j} = \operatorname{score}\left(a, a_{j}\right)&=f_{\text {semantic }}\left(a, a_{j}\right)+f_{\text {time }}\left(a, a_{j}\right)+f_{\text {topic}}\left(a, a_{j}\right).$\\
              
            Where $f_{\text {semantic }}\left(a, a_{j}\right)&=\operatorname{cosine}\left(E_a, E_{a_j}\right)\\
            E_{a} &= \sum_{w \in cls^{a}} TF-IDF\left(w \right) * w2v\left(w \right),$\\
      
            $f_{\text {time }}\left(a, a_{j}\right)=(1 - atanh(|t_s^a - t_s^{a_j}|) * \pi / 2)$\\

            $f_{topic}\left(a, a_{j}\right) = \mathbf{1}\left(Topic^a = Topic^{a_j}\right)$\\
         }
         $a_{max} = argmax(\{s_{a_j}| a_j \in C_a\})$\\
         \eIf{$s_{a_{max}}$ < threshold (1.3 by optimization)}{
            Append $A$ to $Activities$\\
            Search = False
         }
         {
            Add $a_{max}$ to Activity\\
            Remove $a_{max}$ from $R_a$\\
            pre action $a$ = $a_{max}$
         }
         }
   }
%\end{algorithmic}
\end{algorithm}

 \paragraph{Normalized Action Phrase} To avoid the influence of irrelevant words, we extract verb and noun phrases from the original action class text descriptions and perform word lemmatization on them (e.g. "Washing their hands" to "wash hand", "Someone is eating something" to "eat"). \textbf{\textit{Normalized Action Phrase}} will be used for semantic similarity computation in the search step.

 \paragraph{Action Topic} We divide 157 actions into 22 different topics by object type and activity consistency (e.g. "Opening a book" and "Closing a book" are the same topic, "Take clothes from somewhere" and "Someone is dressing" are the same topic). \textbf{\textit{Action Topic}} will be used for the calculation of the topic matching score when searching for the next action.

\subsubsection{Algorithm Implementation}
We have several steps to achieve the greedy algorithm stated in Algorithm \ref{act_algo}.
\paragraph{Step 1} We first sort the action set of the video from early to late according to the start time.

\paragraph{Step 2} The search is started from the earliest starting action after sorting. For the current action $a_{i}$. The candidate set contains the actions that have not been added to any action sequences and started after the start time of the current action $a_{i}$. We calculate the scores $Score(a_i, a_j)$ of all candidates $a_{j}$ according to the following equation, 
\begin{equation}
\operatorname{score}\left(a_{i}, a_{j}\right)&=f_{\text {semantic }}\left(a_{i,} a_{j}\right)+f_{\text {time }}\left(a_{i,} a_{j}\right)+f_{\text {topic }}\left(a_{i,} a_{j}\right). 
\end{equation}

\begin{equation}
\begin{aligned}
f_{\text {semantic }}\left(a_{i,} a_{j}\right)&=\operatorname{cosine}\left(E_{a_i}, E_{a_j}\right)\\
E_{a} &= \sum_{w_{i \in {P}^{a}}} TF-IDF\left(w_{i}\right) * w 2 v\left(w_{i}\right),\\
\end{aligned}
\end{equation}

\begin{equation}
f_{\text {time }}\left(a_{i,} a_{j}\right)=(1 - atanh(|S_t^{a_i} - S_t^{a_j}|) * \pi / 2)
\end{equation}

\begin{equation}
f_{\text {topic }}\left(a_{i,} a_{j}\right) = \mathbf{1}\left({T}^{a_i} = {T}^{a_j}\right)
\end{equation}

Where ${P}_^{a_i}$ is \textbf{Normalized Action Phrase} of action $a_i$, $S_t^{a_i}$ is the start time of $a_i$, 
and ${T}^{a_i}$ is \textbf{Action Topic} of $a_i$. Finally, we select the action that has the highest score from the candidate set.

\paragraph{Step 3} We compare the score of the selected most possible action with the relevance threshold. If the score is higher than the threshold, we consider this action as the next action and add it to the current action sequence. Then we can continue the searching, go back to Step 1 and sort the remaining actions that have not yet formed an action sequence. If there are no actions left, the search is done.

\paragraph{Step 4} Otherwise, if the score is lower than the threshold, it means that all candidate actions are not very relevant to the current action. Therefore, the current action sequence search will be terminated. We then add the current sequence to the activity set and restart the search in the remaining actions. Until there are no remaining actions, the search is finished.

\FloatBarrier

\subsection{Annotation Procedure Design}
\subsubsection{Overview}
\label{appendix:crowdsourcing_overview}
\begin{figure}[!htb]
    \centering
    \includegraphics[width=\linewidth]{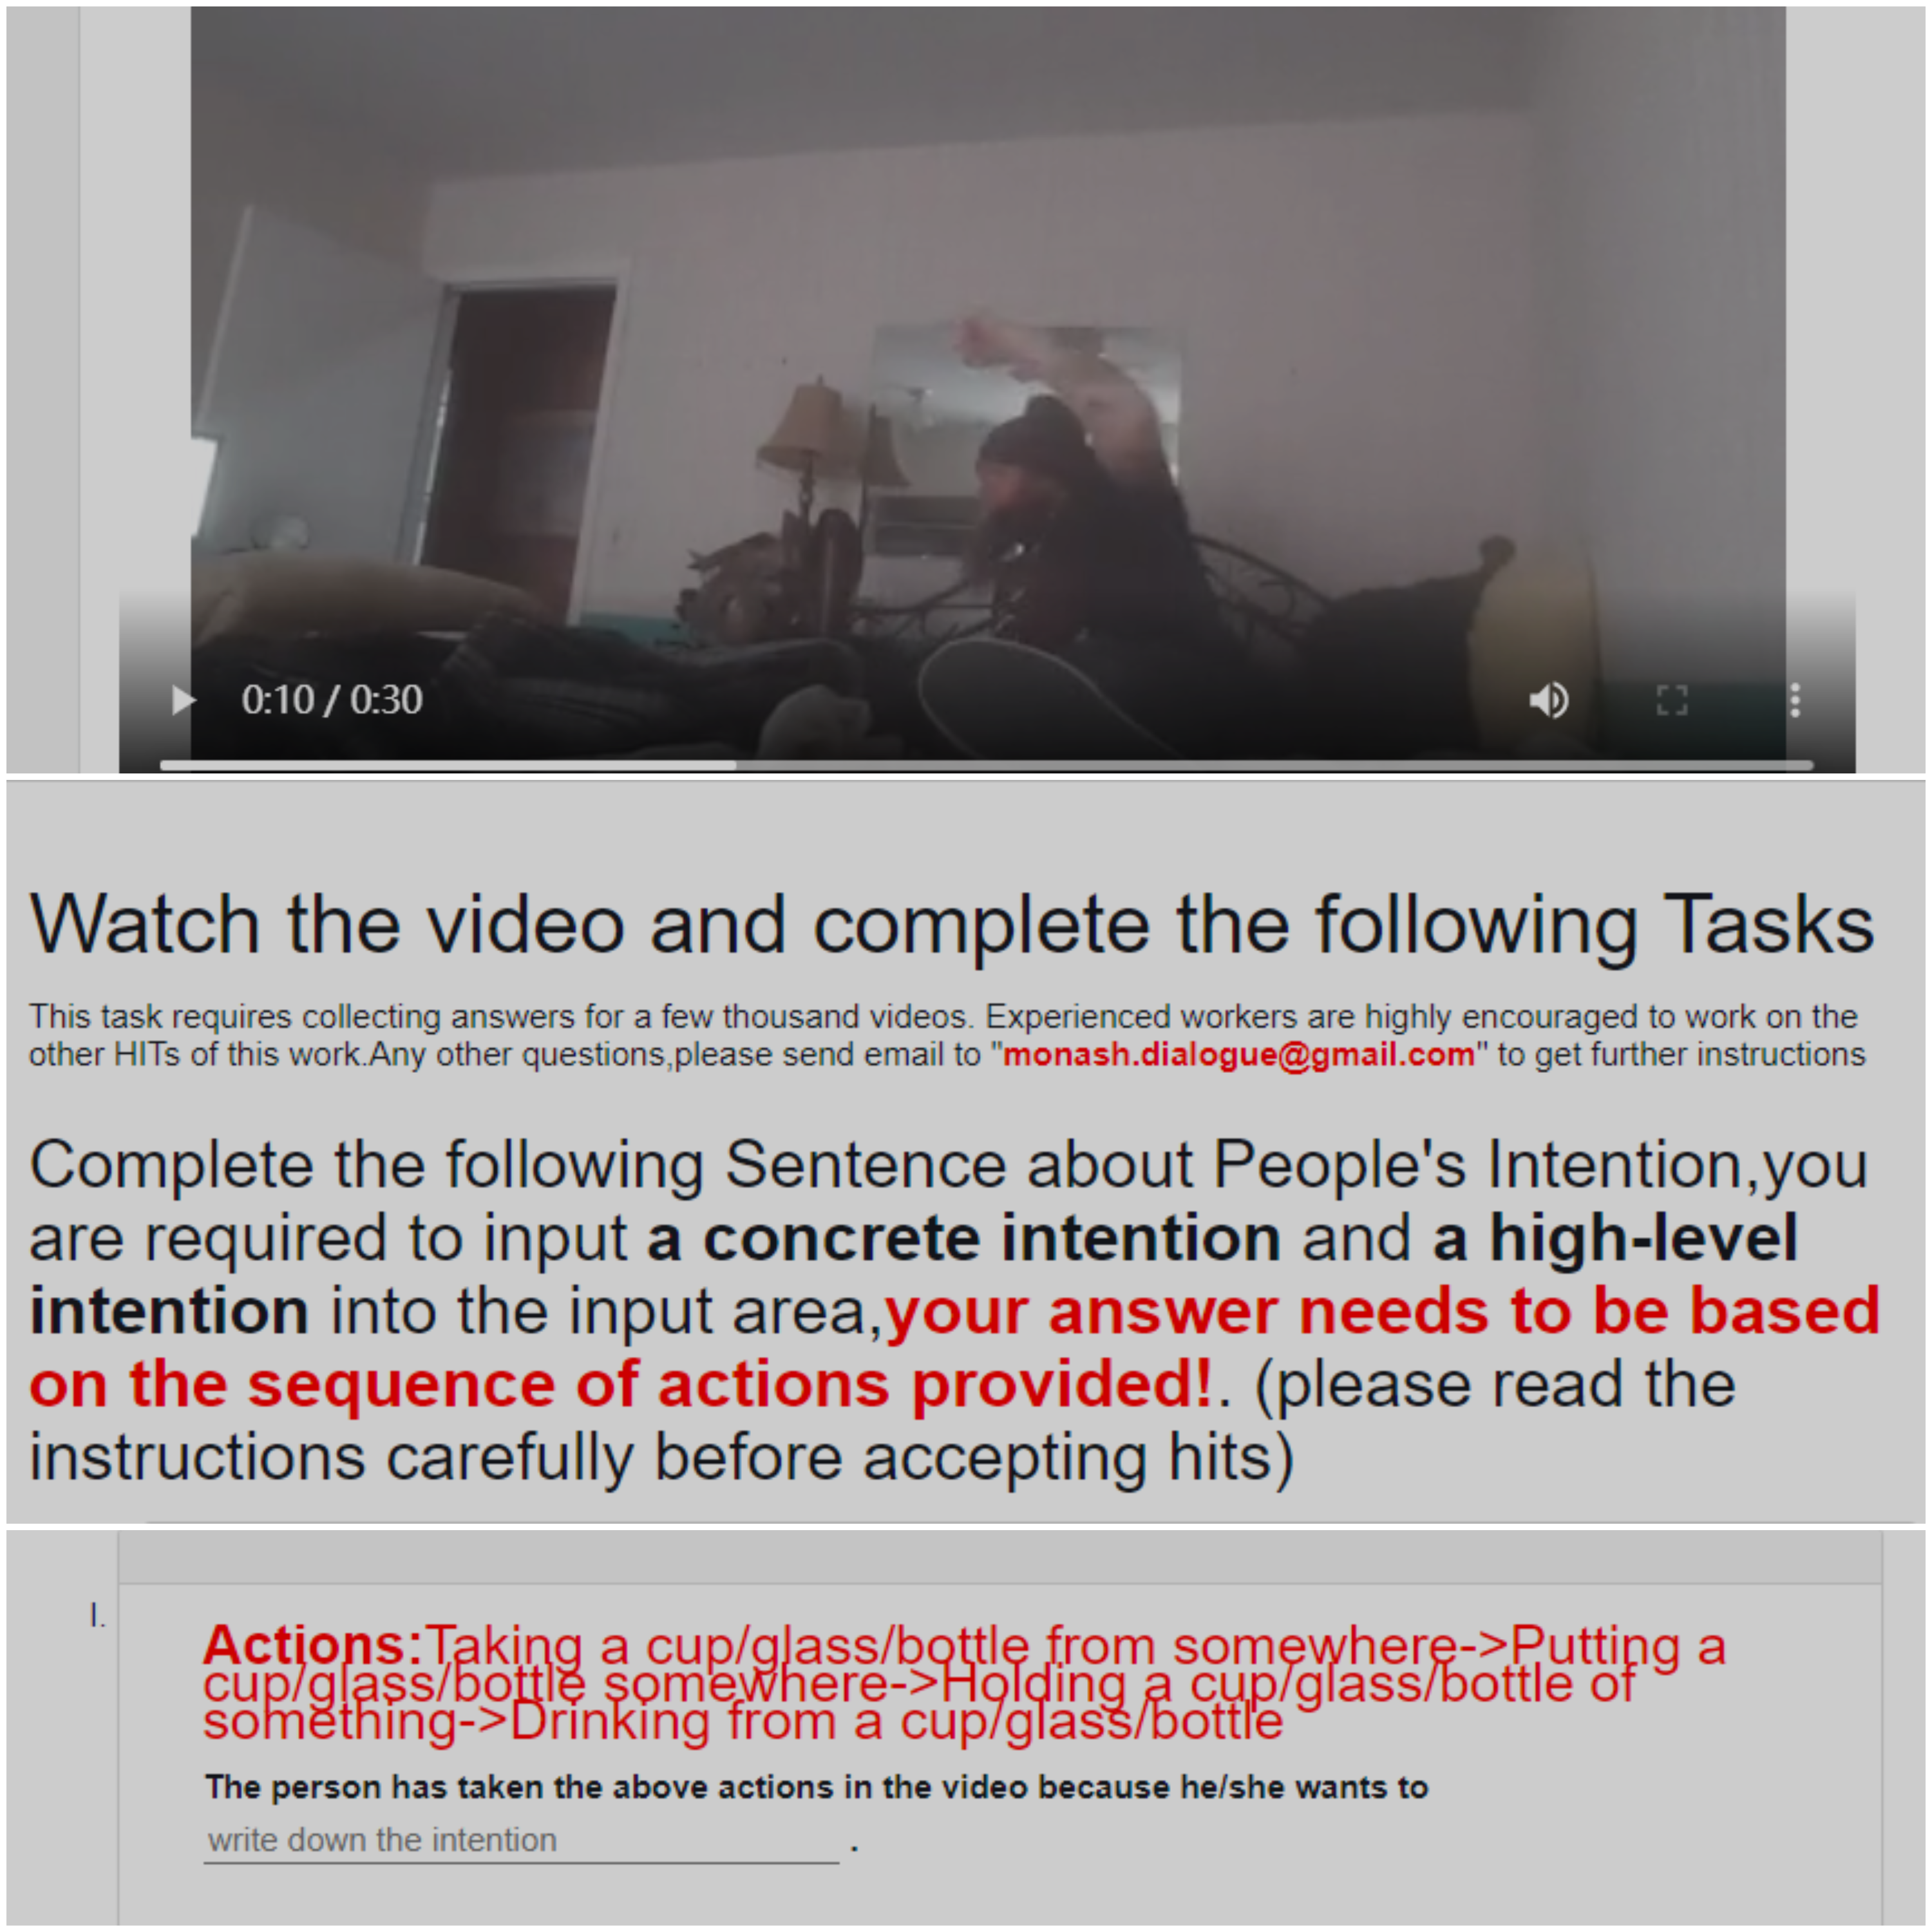}
    \caption{A screenshot of university students annotation interface}
    \label{fig:intent}
\end{figure}
\FloatBarrier

Our dataset firstly needs some experts we choose university students as to annotate the intent of a video based on the content of the video and an action sequence related to the video.

We use the Amazon Mechanical Turk (AMT) platform to build the UI for intent annotation. A screenshot of our interface of this task is given in Figure \ref{fig:intent}. Given a full video and a related sequence of actions, students should describe a concrete intent and a higher-level. The higher-level intent should be generalized from the concrete intent. These are all written in the form of \textit{verb + something}. For example, if the concrete intent is "drink a glass of water", a higher-level intent "quench the thirst" will be right. In our annotation User Interface (UI), students should write their answers in the input area which gives an instruction \textit{write down the intent}.

\begin{figure}[!htb]
    \centering
    \includegraphics[width=\linewidth]{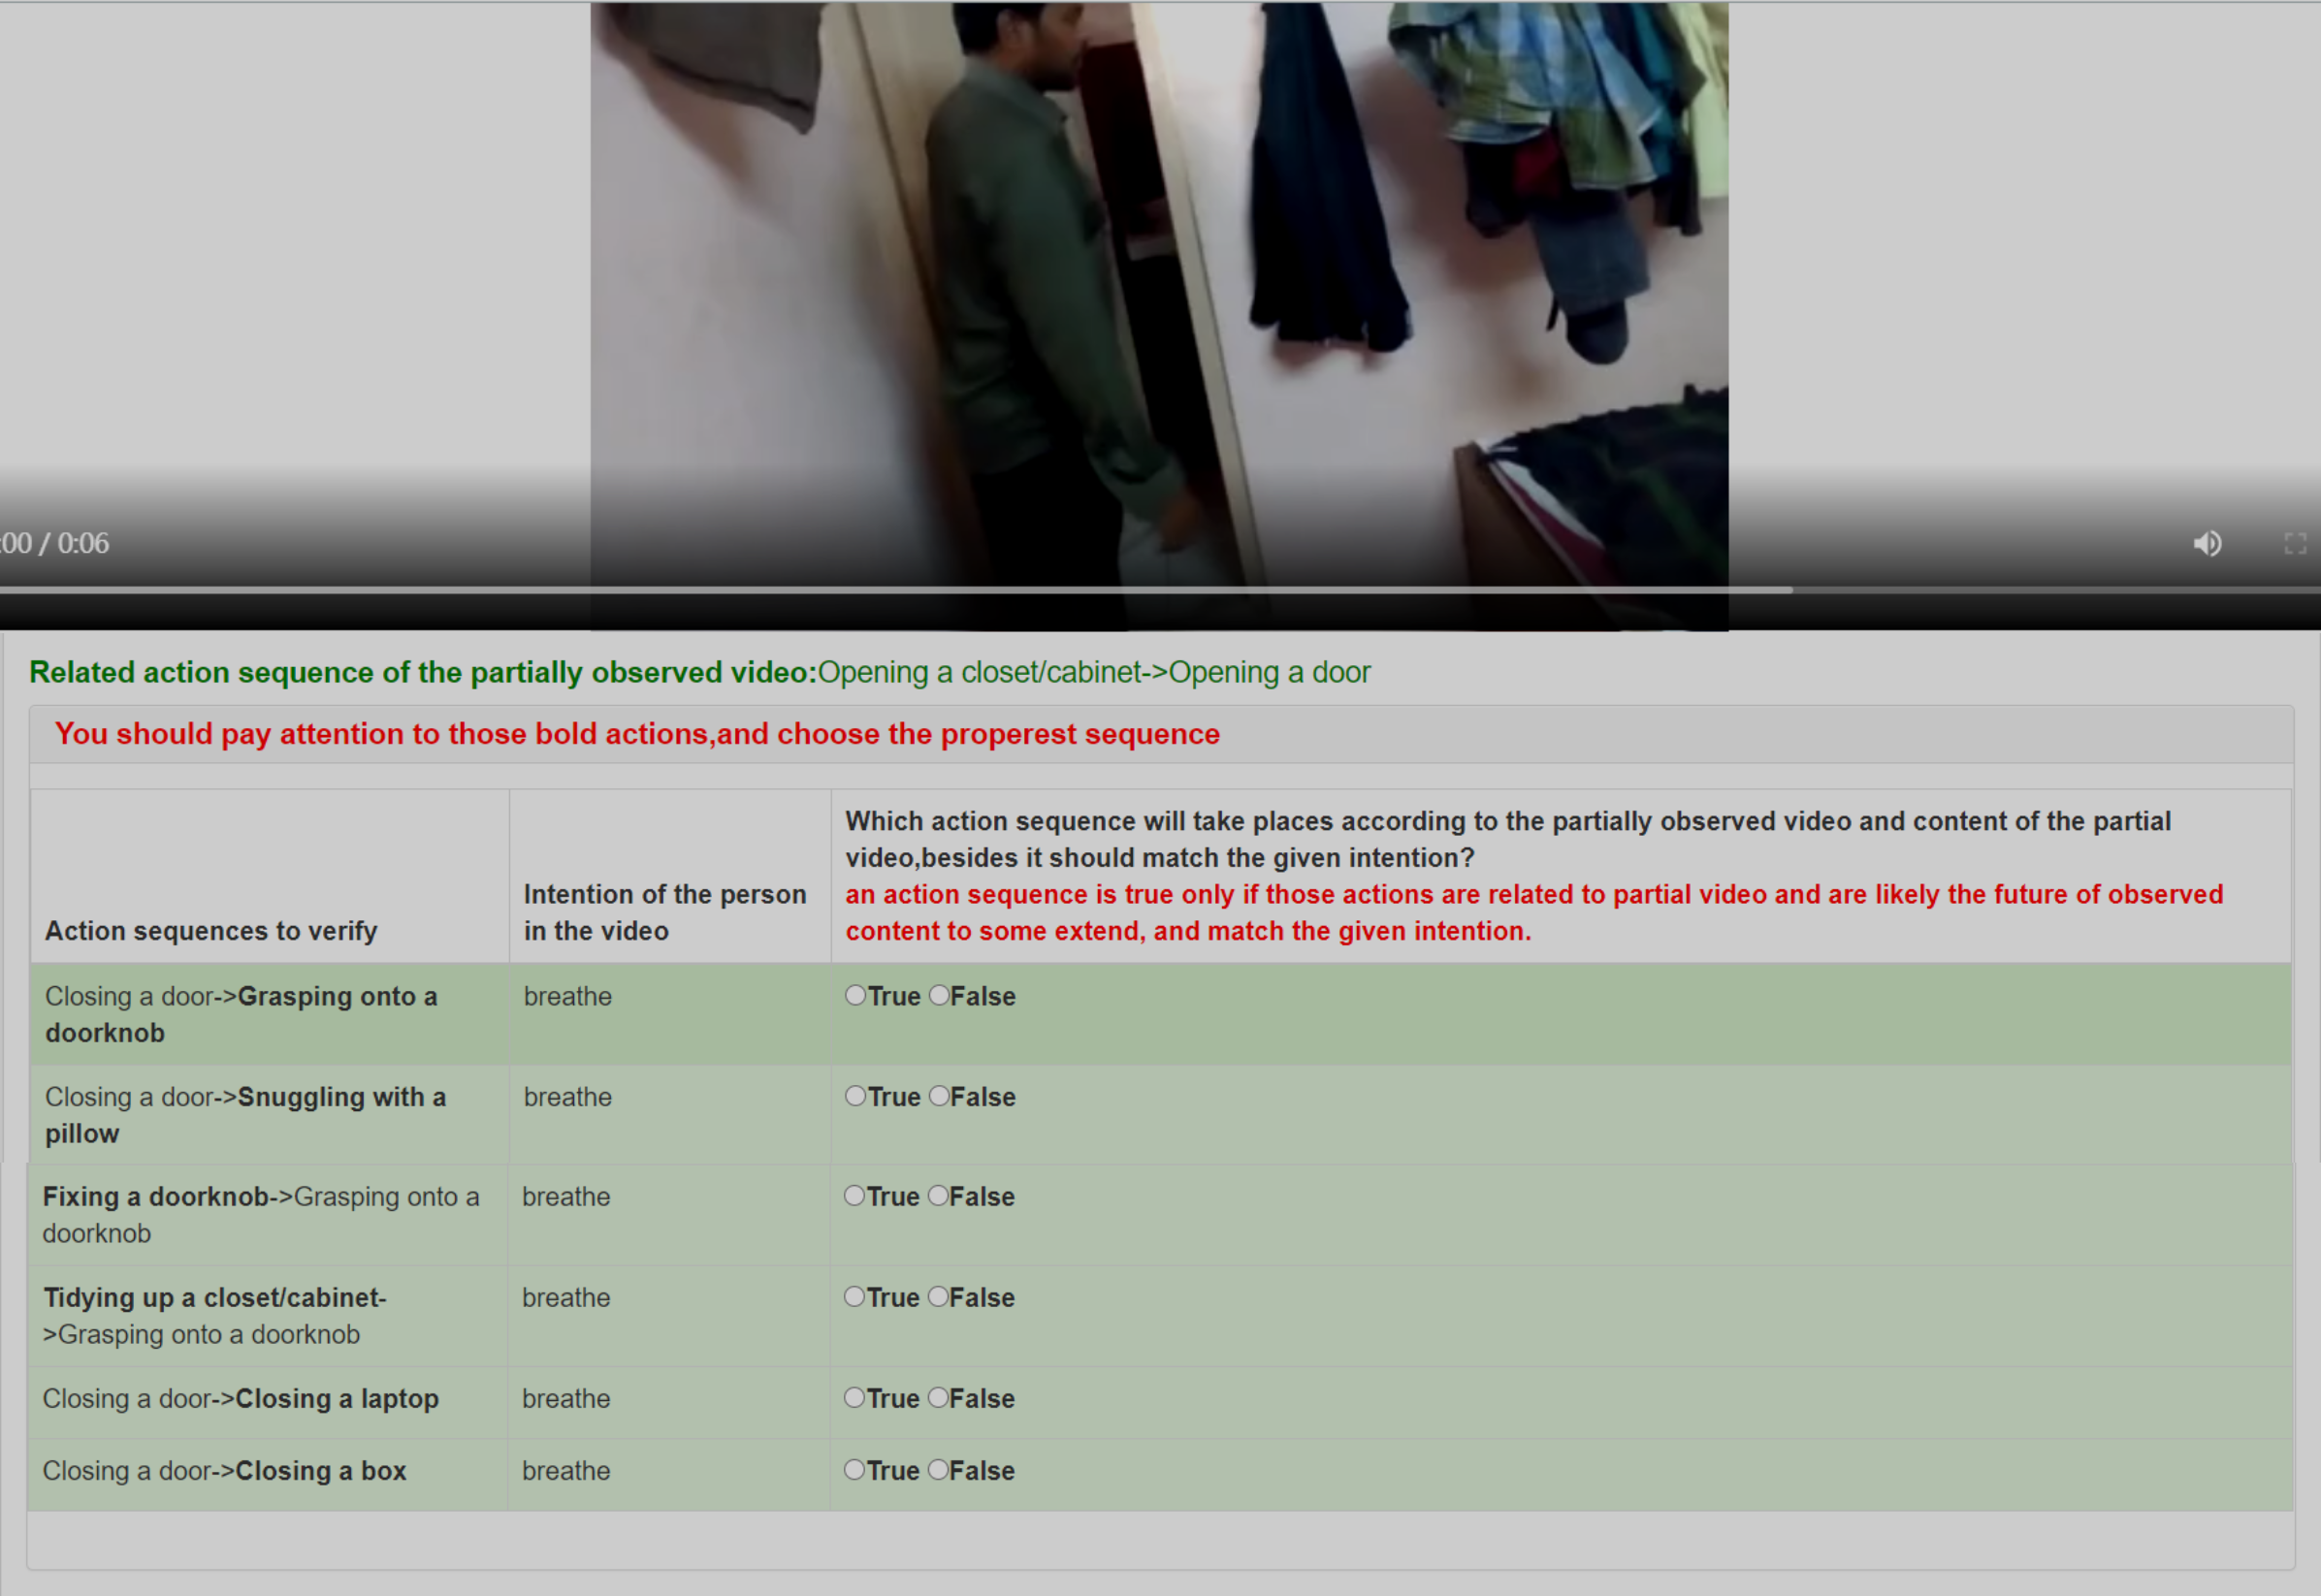}
    \caption{A screenshot of planning task crowdsourcing interface}
    \label{fig:planning}
\end{figure}
\FloatBarrier

When we get a higher-level (future-directed) intent of each video, we could continue designing our crowdsourcing task, which provides turkers with 20\% of the initial video and the related action sequence and the higher-level intent of the full video. Turkers should do some judgments on six action sequences(an original action sequence and five generated ones) based on the above information. They only need to choose "True" or "False" of each action sequence. A screenshot of the task is given in Figure \ref{fig:planning}.

\paragraph{\textbf{Annotation costs}}
 
    Overall we spent about \$2962 for our all annotations task. To obtain the intent of each video, this task was most expensive with an amount of \$2402 for experts. For the intent and action sequence matching evaluation crowdsourcing task, we spent \$300.5 on it. 

\subsubsection{Quality Control}
\label{appendix:crowdsourcing_control}
We apply the quality control for selecting plausible answers from all answer candidates via AMT turkers. Novikova explains the reasons which lead to poor quality data \cite{novikova2016crowd}:
\begin{enumerate}
    \item Task is too complex and instructions are not clear enough.
    \item Financial incentives maybe not attractive enough for turkers to act conscientiously.
    \item Open-ended job designs without a gold-standard reference test may allow them to simply randomly select.
\end{enumerate} 

To address (1), we first adopted worker recruitment and sent emails with our detailed instructions to them, then taught them how to finish our tasks.

To address (2), we raised the payment of each assignment a little and gave those turkers with high-quality results some bonus as encouragement.

To address (3), we set some JavaScript validators to avoid turkers randomly select.

In our procedure of dataset collection, we adopted a complete verification scheme referring to \cite{novikova2016crowd}, which consisted of three main parts:
\begin{enumerate}
    \item \textbf{Worker recruitment} We firstly published some test tasks and invited turkers who were interested in our task to give us their email. Then we chose those turkers according to their results of the test to send them an email containing our detailed instructions and explained the error of their results. In this way, we can confirm those turkers really understand our task. Finally, our recruited turkers would be allocated a qualification called "Master at Sequence Evaluation". Only turkers who obtained the qualification could accept our task hits.
    \item \textbf{Automatic pre-validation} We used two JavaScript validators to avoid turkers randomly select answers or input results copied from our provided sequence. To automatically check the data quality, we add other JavaScript validator checks to the crowdsourcing UI to ensure high quality. To prevent turkers from selecting choices before finishing watching our videos, we set a default limit JavaScript validator, which enables the selection area after the video plays to the end. A new JavaScript validator that restricts turkers from selecting more than one true sequence will help us use some rules to obtain our crowdsourcing results. 
    \item \textbf{Human evaluation of collected data} For the task of intent inference, we asked a group of students,who are not authors as a third party to design a 5-point Likert scales to judge data from crowdsourcing experts, via three criteria: grammaticality, format, and semantic relevance. For the action sequence evaluation process and intent and action sequence matching evaluation process, we made a serial of rules for data collected from turkers to get the final results. Then we randomly sampled 40 videos to ask human experts to give us their results. Finally, we adopted a quality consistency Kappa coefficient \cite{kraemer2014kappa} to evaluate the consistency between the results from turkers and results from the third party.
\end{enumerate}
\paragraph{Quality Evaluation}
In order to judge our crowdsourcing results can be used to construct our dataset, we adopt the Kappa coefficient as a measure for activity planning evaluation task. We randomly select 40 videos in order to ask the third-party experts to finish them just like turkers and get Kappa coefficient of 0.91. The detailed Kappa coefficient of the evaluation task is shown in Table \ref{tab:my_label2}.
% \begin{table}[hbt!]
%     \centering
%     \begin{tabular}{|c|c|c|c|c|}
%     \hline
    
%     \multicolumn{2}{|c|}{\multirow{2}{*}{Setting}}&\multicolumn{2}{c|}{Third party}& \multirow{2}{*}{sum}\\
%     \cline{3-4}
%     \multicolumn{2}{|c|}{}&True&False& \\
%     \hline
%     \multirow{2}{*}{Rules}&True&34&3&37 \\
%     \cline{2-5}
%     &False&4&199&203 \\
%     \cline{1-5}
%     \multicolumn{2}{|c|}{sum}&38&202&240 \\ 
%     \hline
%     \end{tabular}
%     \caption{Detail of Kappa at action sequence evaluation task}
%     \label{tab:my_label1}
% \end{table}

\begin{table}[hbt!]
    \centering
    \begin{tabular}{|c|c|c|c|c|}
    \hline
    
    \multicolumn{2}{|c|}{\multirow{2}{*}{Setting}}&\multicolumn{2}{c|}{Third party}& \multirow{2}{*}{sum}\\
    \cline{3-4}
    \multicolumn{2}{|c|}{}&True&False& \\
    \hline
    \multirow{2}{*}{Rules}&True&37&3&40 \\
    \cline{2-5}
    &False&3&197&200 \\
    \cline{1-5}
    \multicolumn{2}{|c|}{sum}&40&200&240 \\ 
    \hline
    \end{tabular}
    \caption{Detail of Kappa evaluation on intents' alignment with action sequences.}
    \label{tab:my_label2}
\end{table}

    To a certain extent, the results of inter-annotator agreement between third party and turkers,which we get the corresponding Kappa coefficient 0.91,shows that our crowdsourcing data can be used for our evaluation task.
% \begin{table}[h]
%     \scalebox{0.5}{\begin{tabular}{|c|c|c|}
%     \hline
%      Type of Crowdsourcing Task & Action Sequence Evaluation & intent\&Action Sequence Matching Evaluation \\ 
%      \hline
%     Value of Kappa coefficient & 0.8885 & 0.9100 \\ 
%     \hline

%     \end{tabular}}
%     \caption{The value of Kappa on crowdsourcing task}
%     \label{table:kappa}

% \end{table}

\subsubsection{Annotation Rules}
\label{appendix:crowdsourcing_rule}
A set of heuristic rules to determine the final answer to each question are showing blow:

\begin{myRules}
We set five hits for each video, that is to say, we will get five results from five turkers.

\end{myRules}

\begin{myRules}

If more than four of the five results give the same answer, then we adopt the same answer as this sequence's final result. for example, if there is a sequence that at least four turkers select the "True (or False)" option, then we think this sequence is "True (or False)".

\end{myRules}

\begin{myRules}

After the above filtering rule, only three of the five results give the same answer. Then we introduce a third-party human check to judge whether the sequence is true or false. The third party (human expert) should review our videos, then combine the remaining sequences with the results from turkers, finally give their judgment.
\end{myRules}

\begin{myRules}

After the third party finishing their works, we will get most videos that only have one true sequence and five false sequences. We adopt these results of videos as our final dataset. As for others that maybe have more than one true sequence or zero true sequence, we check these videos and decide whether the results of these videos are proper to our task. For the planning task, we only choose the properest sequence as a single choice, so we will remove those videos with zero true sequences and only select one true sequence as a final true sequence for those videos with more than one true sequence. 

\end{myRules}
    
\section{Task Examples}
\label{appendix:task_example}
Figure \ref{fig:examples} displays examples of our task data.
\begin{figure}[htb]
    \includegraphics[width=\linewidth]{diagrams/examples(1).pdf}
    % \makebox[\textwidth]{\includegraphics[width=\paperwidth]{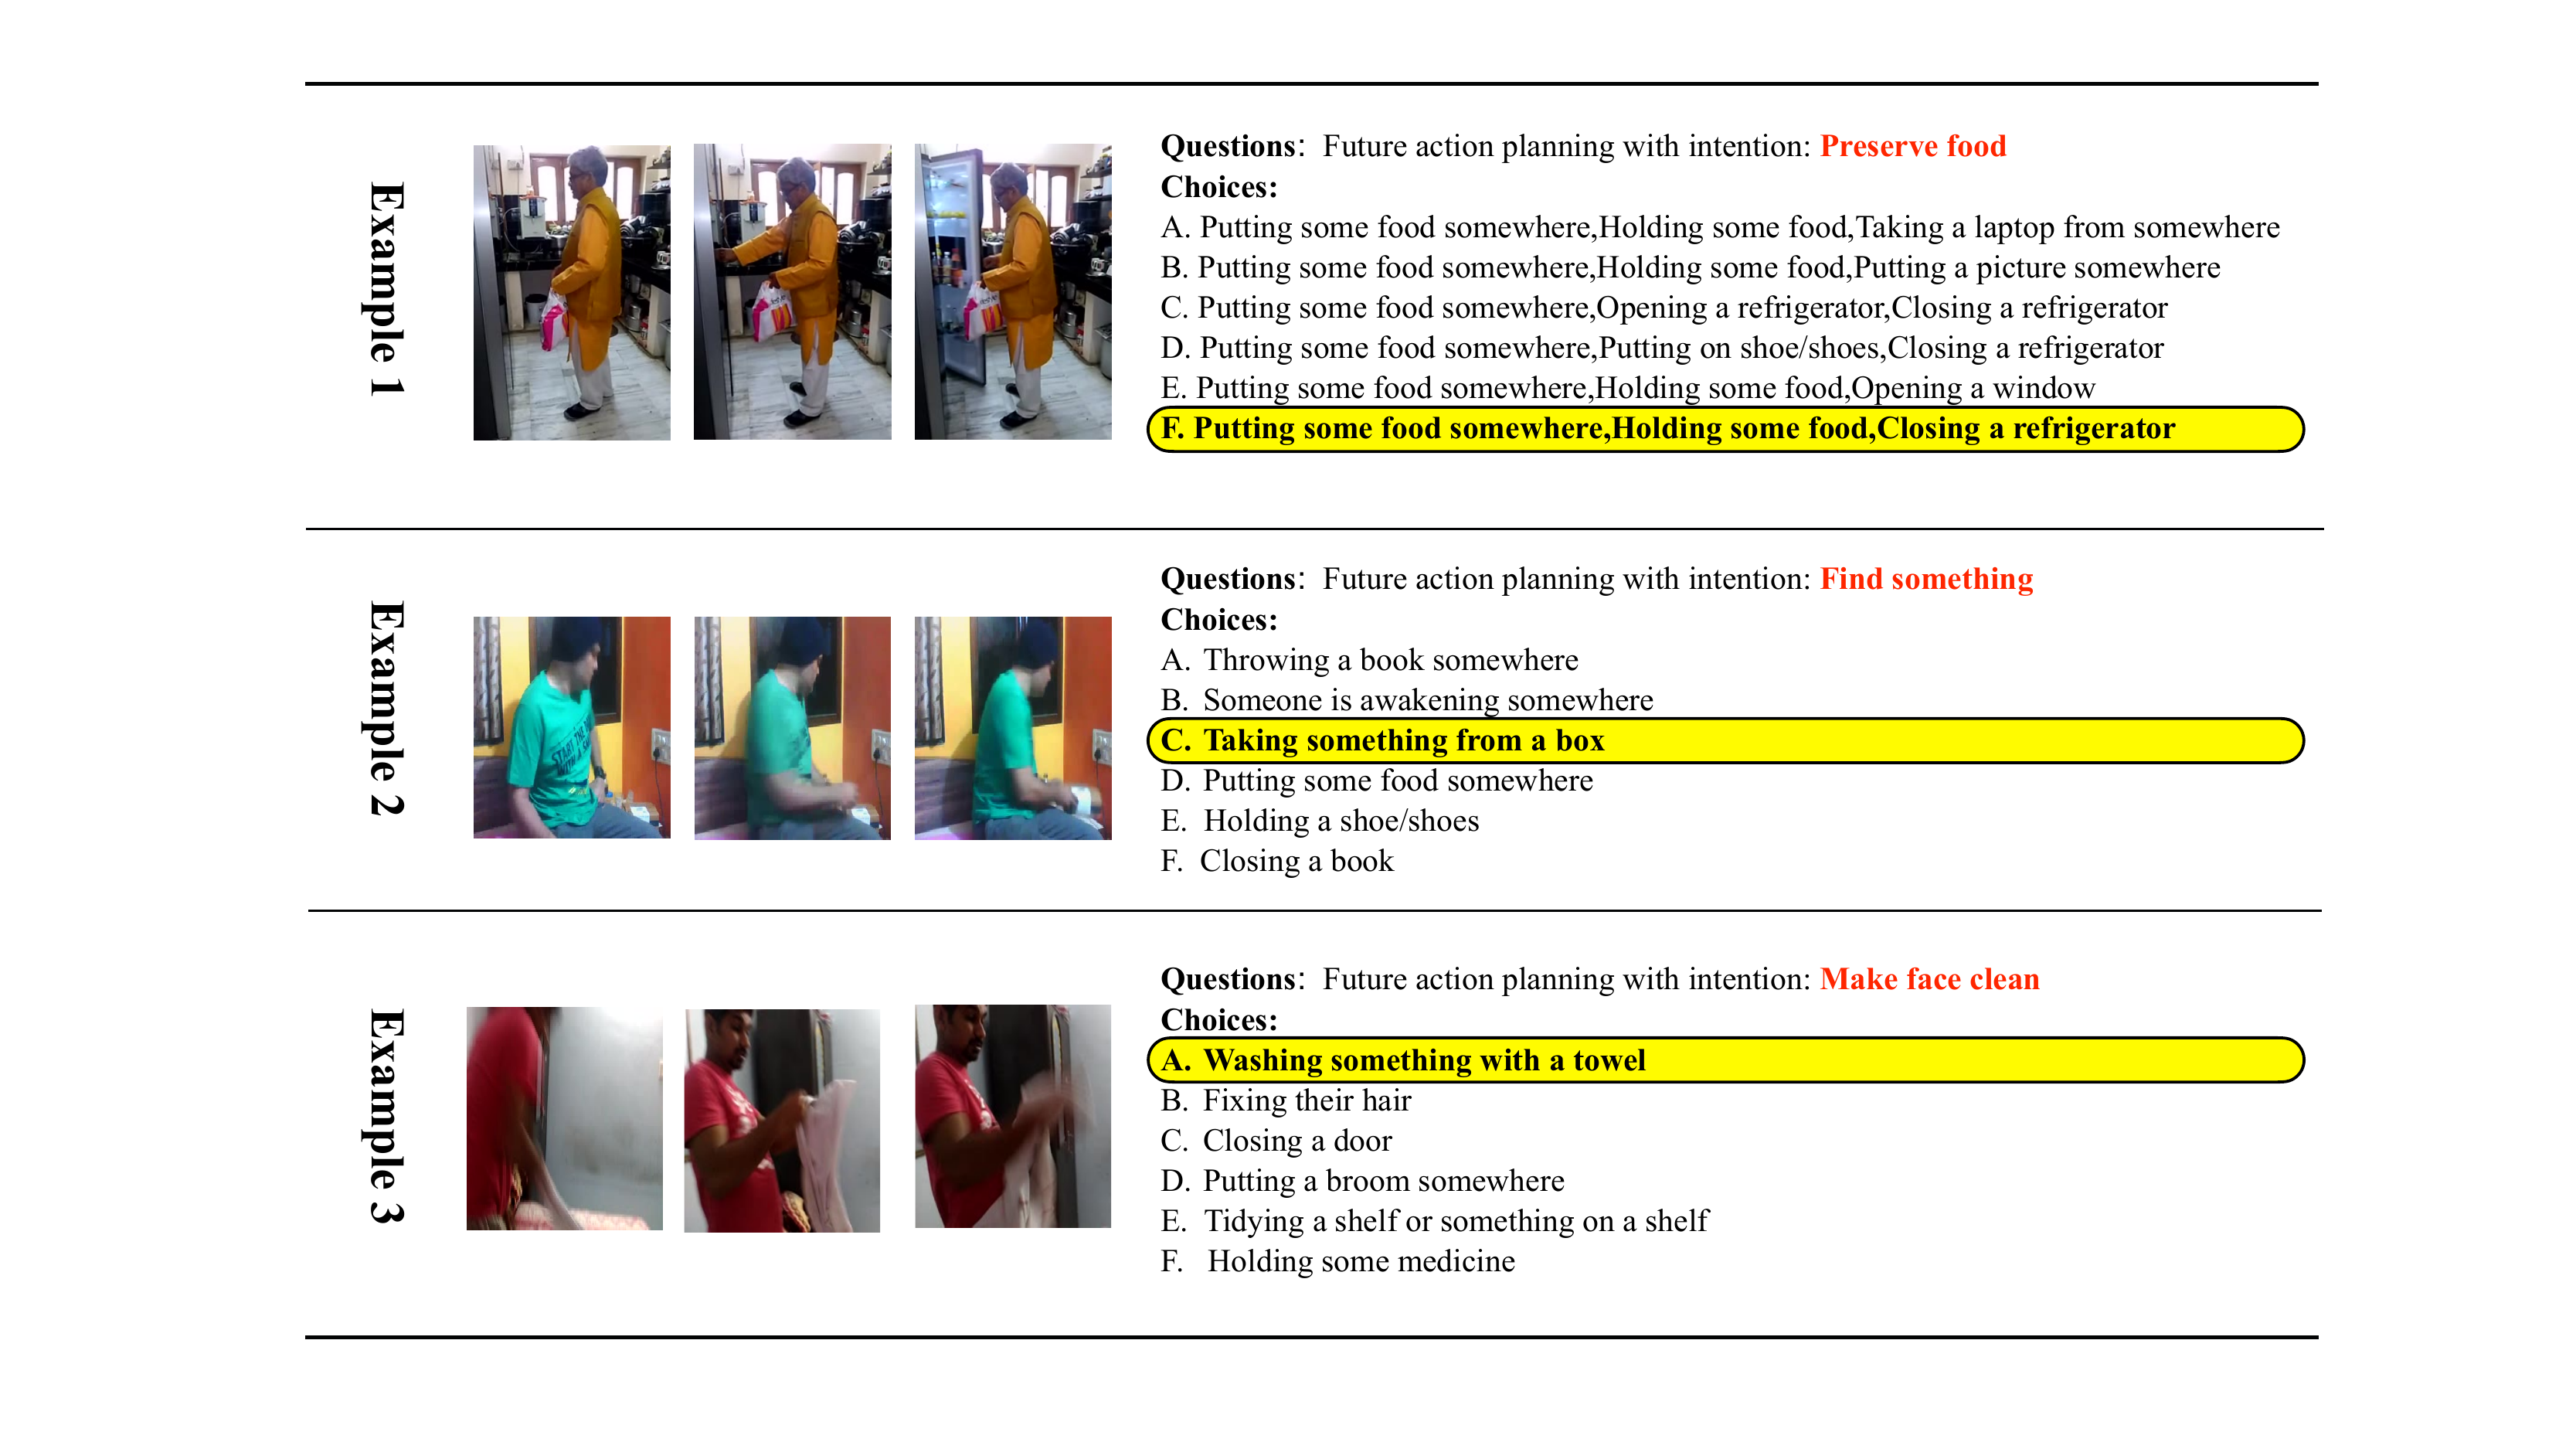}}
    \caption{Examples of \dataset test data.}
    \label{fig:examples}
\end{figure}

\section{Model Details}

\subsection{Deep Generative Models}
\label{appendix:deep_generative}
\subsubsection{Two Stage Planning Model}
%  When fine-tuning \uniVL on the downstream of captioning observed action sequences, we set max frame, mean frames and feature frame rate of the encoded features to 629, 113 and 3, and keep the remaining hyperparameters the same as that on YoucookII~\cite{krishna2017dense}.
 
 Generally, when we encode and decode the action sequence, we treat each action as a whole word instead of a combination of sub-words. For \uniVL caption task, we first use the fine-tuned \itd encoder to extract the features from the input video. To fine tune \uniVL, we set max frame, mean frames and feature frame rate of the encoded features to be 629, 113 and 3. The other details are the same as the caption task on YoucookII \cite{krishna2017dense} originally reported in \uniVL. Our text input of \uniVL is the observed action sequence till activity observation end time, which is taken as the caption. For the video input, we use \itd encoded video frames aligned with activity observation end time. \uniVL randomly masked text inputs and video inputs to predict given captions. We fine tune the model for 40 epochs on 2 Nvidia Tesla V100 GPUs to achieve the best results. During generation, we follow \cite{luo2020univl} to generate captions only based on the encoded video features.
 
For \prophetNet translation task, we follow all the settings in \cite{qi2020prophetnet}. We change the original vocabulary of the model in order to make each action be encoded as a subword, which reduce the generation randomness. More specifically, we replace $[unusedXX]$ with actions labels, where $XX$ represents a vocabulary ID. For example, we replace $[unused255]$ with the action label $SomeoneIsEatingSomething$. The encoder inputs of \prophetNet are intents, \uniVL generated observed action sequences. The decoder inputs are future action sequences. By fine-tuning the model from \prophetNetEN pretrained checkpoint for 50 epochs on 2 Nvidia Tesla V100 GPUs, we choose the best model based on the validation loss. We follow the same parameters and hyperparameters stated in the original \prophetNet experiment.
From what the best model we trained, there is no random word besides pre-added action labels during model generation. Hence, no post-processing step is required.

\subsubsection{Intents Augmented Action Forecasting Model}
We implement the model architecture based on the details in \cite{ng2020forecasting}, where we have intents and \itd features of observed video frames as the encoder inputs. We let the model to forecast both the observed action sequences and future action sequences. While we index the text input, we additionally index each action as a whole word, which will reduce the forecasting randomness. the During generation, we let the model forecast action sequences with limiting the length. Instead, the generation is stopped when the model forecasts the special token \textit{EOS}. As most of the parameters are not mentioned in \cite{ng2020forecasting}, we set input size of the encoder as $1024$, hidden size of the encoder as $512$; hidden size of the decoder as $512$, output size of the decoder as $512$; hidden size of the decoder with attention as $512$, output size of the decoder with attention as $160$. The training procedure is under the setting of $0.5$ learning rate and $0.5$ teaching forcing ratio. We train the model for 50 epochs to get the best model on 2 Nvidia Tesla V100 GPUs.

\subsection{Multimodal Knowledge Base}
\label{appendix:mkb}
\input{mkb}

\subsection{Explainable Neurosymbolic Planning}
\label{appendix:explainable_planning}
We have designed the retrieval process into two stages. In the \textbf{First Stage}, to effectively obtain top-50 candidates, we extend the traditional \bmTF algorithm to our setting, where we use \uniVL \cite{luo2020univl}, a video-language pre-trained model for both video language understanding and generation tasks, to predict observed action set $A_{q} = \{a_{1},...a_{q_n}\}$ from frame-level visual feature sequence as query. The action sequences in MKB are treated as documents to be retrieved by bag-of-actions $A_{q}$. The \bmTF score $s_{bm25}(KB, A_{q})$ is computed based on the query actions appearing in each action sequence, 
\begin{equation}
\resizebox{0.95\hsize}{!}{$
\operatorname{s_{bm25}}(KB, Q)=\sum_{i=1}^{n} \operatorname{IDF}\left(a_{i}\right) \cdot \frac{f\left(a_{i}, KB\right) \cdot\left(k_{1}+1\right)}{f\left(a_{i}, KB\right)+k_{1} \cdot\left(1-b+b \cdot \frac{|KB|}{\text { avgdl }}\right)}
$}\end{equation}
where $KB$ is referring to all action sequences in the KB, $avgdl$ is the average length of all action sequences,  and $k_{1}$, $b$ are hyperparameters. Besides using \bmTF to match the initial action sets, we add a text aligner using an embedding-based retrieval method to align the goal states(intents). This uses a \sbert \cite{reimers-2019-sentence-bert} to encode MKB intent and query intent to get their embeddings and then use cosine similarity to compute their similarity score $s_{intent}(KB, Q)$, which will be combined with \bmTF to get $s_1$ to rank the candidates,
    \begin{equation}
    s_1 = \epsilon * \operatorname{s_{bm25}}(KB, Q) +  (1 - \epsilon) * \operatorname{s_{intent}}(KB, Q)
     \end{equation} 
 
In the \textbf{Second Stage}, to get a more accurate ranking and take the top-k references, we apply Ordered Temporal Alignment Module (OTAM) \cite{cao2020few} to leverage the temporal order information via \itd visual features,
\begin{equation}
 s_{align} = 1  /  (1 + D_{otam})
\end{equation}  
where the alignment score $s_{align}$ is computed based on 
the distance measure with OTAM, which is a variant of the Dynamic Time Warping (DTW) algorithm in the field of video sequences. This method measures the distance between two videos by aligning their frames while preserving temporal ordering. Unlike DTW having a path aligning the two videos from start to end, it relaxes the boundary condition to find a path with flexible starting and ending positions while maintaining continuity and monotonicity. $D_{otam}$ is the best alignment score on the frame-level distance matrix of query video and MKB candidate activity video. Where the distance matrix is computed based on \itd extracted feature sequences.

To find the sequence that contains the possible unseen actions, we add some rules. The rule score $s_{rule}$ is composed of two binary indicators $s_{last}$ and $s_{len}$,

\begin{equation}
     s_{rule} = \underbrace{I\left[a^{r}_{t} \notin\mathcal{A}_{q}\right]}_{s_{last}} + \underbrace{I\left[|{r}| > \mathcal|\mathcal{A}_{q}|\right]}_{s_{len}}, \\
\end{equation}
where the first indicator $s_{last}$ measures whether the last action $a^{r}_{t}$ of the retrieved fact $r$ is not in the query action set $A_{q}$, and $s_{len}$ measures whether the length of the retrieved fact $r$ is greater than the number of actions in the query. \\The final score $s_{rank}$ is computed by combining the initial retrieval score  $s_1$ with the visual alignment score $s_{align}$ and $s_{rule}$,
\begin{equation}
    s_{rank} = \alpha * s_{1} + \gamma * s_{align} + \delta * s_{rule} 
    \label{equation:retrieval_final_score}
\end{equation}

For the \textbf{Probabilistic Reasoning} process, we fit Time-warped edit distance (TWED) to visual feature sequences. Like edit distances, TWED is a dynamic programming approach that counts the minimum number of operations required to transform one sequence to another, and like dynamic time warping, it introduces a so-called stiffness parameter $\upsilon$, controlling its 'elasticity. In our setting, we leverage the cosine distance between visual features to measure the cost that transforms one feature into another. Finally, the minimum transform cost will be used to compute the sequence similarity between the retrieved sequence and the visual feature sequence of each choice.\\
\textbf{Parameters}
For our \bmTF function in the first retrieval stage, the parameter $k_{1}$ is 1.5 and  $b$ is 0.75, as for the intent aligner, $\epsilon$ is set to 0.2. In the re-ranking stage, the coefficients $\alpha, \gamma$ and $\delta$ in the final rank score $s_{rank}$ are set to 1, 1 and 0.2. In the answer selection stage, the number $k$ of the retrieved sequence is set to be 10.

\section{Additional Experiments}
%\paragraph{Which visual representation is better, low-level visual features or action labels?} 

\subsection{Comparison of retrieval quality.}
\label{appendix:rq2}
\begin{table*}[htb]
\vspace{-1ex}
\begin{center}
%\vspace{-1ex}

 \adjustbox{max width=\textwidth}{\begin{tabular}{|c|c|c|c|c|c|c|c|c|c|}
\hline
 \multirow{2}{*}{setting} & \multicolumn{7}{c|}{Quality} & \multicolumn{2}{c|}{Diversity} \\ \cline{2-10} 
\multicolumn{1}{|c|}{} & precision & \multicolumn{1}{c|}{recall} & \multicolumn{1}{c|}{seq-item-acc} & seq-hits@5 & seq-hits@10 & BLEU-1 & BLEU-2 & \multicolumn{1}{c|}{Dist1} & Dist2 \\ 
\hline
\AttentionGRU  &15.45&11.65&2.67&0.00&0.00&8.69&1.99&9.79&26.99\\\hline
\UniVLProphetNet &38.71&30.73&11.06&2.48&5.79&29.60&13.71&15.45&35.37 \\\hline
\RetrievalScoring
&\textbf{41.16}&\textbf{35.68}&\textbf{11.26}&\textbf{26.45}&\textbf{34.71}&\textbf{34.05}&\textbf{15.85}&\textbf{28.02}&\textbf{62.55}\\\hline
\prophetNet
&- &- &-  &-  &-  &- &- &- &-\\\hline
\uniVL
&- &- &-  &-  &-  &- &- &- &-\\\hline
\end{tabular}}
\caption{Comparison of top-10 action sequences of all systems.}
\label{appendix:table: Comparison of top-K action sequences of two baselines}
\end{center}
% \vspace{-3mm}
\end{table*}

\begin{table*}[htb]
\vspace{-1ex}
\begin{center}
%\vspace{-1ex}

 \adjustbox{max width=\textwidth}{\begin{tabular}{|c|c|c|c|c|c|c|c|c|c|}
\hline
 \multirow{2}{*}{setting} & \multicolumn{7}{c|}{Quality} & \multicolumn{2}{c|}{Diversity} \\ \cline{2-10} 
\multicolumn{1}{|c|}{} & precision & \multicolumn{1}{c|}{recall} & \multicolumn{1}{c|}{seq-item-acc} & seq-hits@5 & seq-hits@10 & BLEU-1 & BLEU-2 & \multicolumn{1}{c|}{Dist1} & Dist2 \\ 
\hline
\AttentionGRU  &7.35&10.38&1.15&0.00&0.00&4.10&0.88&6.33&9.52\\\hline
\UniVLProphetNet &21.59 &15.59&9.26&10.00&\textbf{16.86}&12.50&3.58&32.55&58.54 \\\hline
\RetrievalScoring
&20.78&\textbf{22.06}&8.50&5.88&7.45&19.60&\textbf{7.01}&37.91&66.85\\\hline
\prophetNet
&21.35 &19.75 &8.12  & \textbf{12.75} & 16.08 & 18.66 & 5.52 &51.96 &81.93\\\hline
\uniVL
&\textbf{23.67} &22.02 &\textbf{9.71}  &  9.61& 10.59 & \textbf{20.52} & 6.52 &47.10 &77.42\\\hline
\end{tabular}}
\caption{Comparison of top-10 future sequences of all systems.}
\label{appendix:table: Comparison of top-K future sequences of two baselines}
\end{center}
% \vspace{-3mm}
\end{table*}

\label{appendix:rq2}
% \begin{table}[htb]
% \vspace{-1ex}
% \begin{center}
% \caption{\AttentionGRU Observation Action Sequence Evaluation Results}
% \vspace{-1ex}
%  \adjustbox{max width=\textwidth}{\begin{tabular}{|c|c|c|c|c|c|c|c|c|c|}
% \hline
%  \multirow{2}{*}{setting} & \multicolumn{7}{c|}{Quality} & \multicolumn{2}{c|}{Diversity} \\ \cline{2-10} 
% \multicolumn{1}{|c|}{} & precision & \multicolumn{1}{c|}{recall} & \multicolumn{1}{c|}{seq-item-acc} & seq-hits@5 & seq-hits@10 & BLEU-1 & BLEU-2 & \multicolumn{1}{c|}{Dist1} & Dist2 \\ 
% \hline
% \AttentionGRU  &10.98&7.11&4.22&0.20&0.20&7.29&2.92&11.11&48.82\\\hline
% \end{tabular}}
% \end{center}
% \vspace{-3ex}
% \end{table}

In Table \ref{appendix:table: Comparison of top-K action sequences of two baselines} and Table \ref{appendix:table: Comparison of top-K future sequences of two baselines}, we use the precision, recall, sequence-item classification accuracy\cite{ng2020forecasting}, sequence-item hit rate, seq-hits@10, BLEU-1, and BLEU-2 to measure the quality of top-10 full sequences and future sequences obtained by baselines. In terms of the action-level diversity, we report Dist1 and Dist2 that are used in \cite{distinct}.

\begin{itemize}
\item Sequence item classification accuracy:  it evaluates the exact action matching in the predicted action sequence with ground truth, which counts how many times the action in the predicted sequence matches the ground truth in the exact position. For top-10 sequences, we calculate the mean accuracy of all sequences.
\item Precision and recall: The precision and recall do not consider the order of ground truth. They both treat the actions inside the sequence as a unified set. The precision of top-10 sequences is computed by averaging the precision of each sequence, which measures the number of true actions over the number of total actions in the sequence. Here, we define the true action as the action that occurred in the ground truth. Similarly, the recall of top-10 sequences is also computed by averaging all sequences' recall, which is a measure of the true actions over the number of ground truth actions.
\item Seq-hits: The seq-hits is used to measure the sequence exact matching, which is calculated as the number of examples whose top-k sequences include the ground truth sequence, and we report the seq-hits@5 and seq-hits@10 accordingly. As for retrieval-based baseline, we only consider the in-domain situation where the ground truth sequences have also appeared in the knowledge base.
\item BLEU:  We use the standard BLEU
score that is widely used in the Machine Translation Field and fit it to our situation by computing action-level match.
\item Dist: We report Dist1 (Distinct-1) and Dist2 (Distinct-2) definition proposed in the \cite{distinct}, to measure the diversity of action sequences, which is used to compute the number of distinct n-gram of top-10 sequences.
\end{itemize}

%\begin{table}[h]
%\centering
%\caption{Performance of action recognition methods.}
%\vspace{-1ex}
%\label{table: Comparison of action recognition methods}
%\scalebox{0.7}{\begin{tabular}{|c|c|c|c|c|}
%\hline
%\multirow{2}{*}{Method} & \multicolumn{4}{c|}{Action Recognition} \\ %\cline{2-5} & Acc@1 & \multicolumn{1}{c|}{Acc@5} & %\multicolumn{1}{c|}{Rec@1} & Rec@5 \\ \hline
%\prototype& 21.96 & 18.84 & 9.09 & 34.73\\
% \slowFast& 34.48& 21.77 & 13.34 & 39.69 \\
%\itd & 36.22 & 24.35 & 14.83 & 45.13 \\ \hline
%\end{tabular}}
%\end{table}
\subsection{Factors Influencing Retrieval Quality}
\label{appendix:retrieval_quality}

\paragraph{Effect of action recognition. }

For our MKB retrieval module of \RetrievalScoring, we compare models that only use low-level visual features (neural representations) to search, include video-level feature search and frame-level feature alignment, and the models using action labels (symbolic representations) predicted by an action recognition model based on neural representations to do text retrieval (\prototype\_\bmTF, \itd\_\bmTF, \slowFast\_\bmTF, and \uniVL\_\bmTF). Details are as follows:

\begin{itemize}
    \item \textbf{Methods only use low-level visual features: } These methods directly use the low-level visual features of the input video as a query to do similar video retrieval. Where video-level feature search calculates the cosine similarity of video-level features between the input video and the MKB activity videos to score the facts in the MKB, and the frame-level feature alignment leverages OTAM to compute the similarity between frame-level feature sequences.

    \item \textbf{Methods use action recognition and text retrieval: } We identify the actions of the input video and then use text retrieval methods to retrieve the most relevant action sequences and their corresponding videos. We compare the \prototype\_\bmTF, \itd\_\bmTF, \slowFast\_\bmTF, and \uniVL\_\bmTF to do the action recognition. In the \prototype\_\bmTF, we use the mean-pooling vector of input video as the query, to search in the 157 visual prototypes from KB to find the top-5 neighbors. In \itd\_\bmTF and \slowFast\_\bmTF approaches, an action probability distribution can be obtained by \itd and \slowFast\cite{fan2020pyslowfast}. Based on this, we filter the actions in top-5 by the threshold. As for \uniVL\_\bmTF, it can learn the observed action sequence by video caption. The textual action set will be considered as the query of the \bmTF.
\end{itemize}

From Table \ref{table:Results of knowledge base retrieval}, we find that leveraging recognition models can better improve all metrics of top-10 sequences compared to the low-level feature search. We also report the results obtained by using the ground truth actions as the query of \bmTF, which can be served as a soft upper bound for the action recognition-based method. The result shows that the retrieval module using the ground truth has a significant improvement. Therefore, the accuracy of the recognition model has a great influence on the final result. 
\paragraph{Effect of re-ranking by visual feature alignment and forecasting rules in Second Stage Retrieval. } We observe that using visual alignment scores combined with original \bmTF scores to re-rank the top-50 results of \bmTF-initial retrieval yields better performance. It is shown in Table \ref{table:Results of knowledge base retrieval} that using visual features to re-ranking the results performs better than the methods that only use \bmTF to rank the retrieved results. We also find that adding some forecasting rules can help the process of re-ranking and improve the recall, seq-item-acc, and BLEU scores. Especially under the assumption that the action recognition is completely correct, adding this rule score can significantly improve the hit rate.

\paragraph{Usefulness of intent. }  We study the effect of adding intent in the retrieval process. It has been shown in Table \ref{table:Results of knowledge base retrieval} that leveraging high-level intent can improve the quality and diversity of retrieved results.  Compared to our \uniVL\_\bmTF + OTAM\_Rule model, adding the intent aligner contribute to an increase of 9.93\% in precision from 37.44 to 41.16, and 11.04\% in the seq-item-acc from 10.14 to 11.26. The reason might be that the lack of discriminative action information in the partially observed videos and the error rate of initial action recognition can affect the quality of retrieval results. While adding the high-level intent as the goal of the input video and using an intent aligner to search for action sequences with similar intent can alleviate the problem of action uncertainty and error in action recognition models, thus making the search results more accurate.

\subsection{Details of different similarity methods in probabilistic reasoning}
\label{appendix:anwer_score}
The specific implementation of the optional similarity measure in our reasoner is as follows. When only using the index of action class, $L_{2}$ metric is adopted to compute the pairwise distance in the matrix, and in the other feature-based settings we use cosine similarity matrix. In the Mean method, we compute sequence-level similarity through doing mean-pooling on the cosine similarity matrix of the retrieved action sequence and ground truth action sequence. In the Max-pooling, we use max-pooling the final score averaging the maximum score of each row in the distance matrix, so that each action is matched to the most similar action in the other sequence. While max-pooling neglects the temporal order of the action sequence, We use a variant of the DTW algorithm and OTAM to explicitly leverage the temporal ordering information to compute the alignment score on the action-level distance matrix. TWED is a distance measure for discrete time series. We use the pairwise cosine distance as the edit distance between two actions.

\subsection{\RetrievalScoring with ground truth observed sequence}
\label{appendices:nsp_gt_ob_seq}
We conduct additional experiments about our \RetrievalScoring baseline to do retrieval using the ground truth observed actions of input video instead of recognition model prediction results. Table \ref{table:Accuracy of NSPlan with gt on full test data.} has shown that the accuracy of *gt\_\RetrievalScoring on the full multi-choice question
test set goes up to 81.37\%, which can be seen as an upper bound of \RetrievalScoring with perfect action recognition model. And in Table \ref{table:Accuracy of NSPlan with gt on seen data and unseen data.} the accuracy of  *gt\_\RetrievalScoring can reach 94.21 \% in seen data.
 
 \begin{table}[h]
  \vspace{-1mm}
 \centering

 \vspace{-1ex}

 \adjustbox{max width=\columnwidth}{
 \begin{tabular}{|c|c|c|}
 \hline
 \row{Method} & \RetrievalScoring & *gt\_\RetrievalScoring \\ \hline
   Full Accuracy(\%) &63.72 & 81.37\\\hline
 \end{tabular}}
  \caption{Accuracy of \RetrievalScoring with gt on seen data, unseen data, and full test data.}
  \label{table:Accuracy of NSPlan with gt on full test data.}
 \vspace{-3mm}
 \end{table}
 \\

  \begin{table}[h]
 \centering
 \adjustbox{max width=\columnwidth}{
 \begin{tabular}{|c|c|c|}
 \hline
 \row{Method} & \RetrievalScoring & *gt\_\RetrievalScoring \\ \hline
 Seen Accuracy(\%) & 65.28 & 94.21\\\hline
  UnSeen Accuracy(\%) & 63.23  & 77.37  \\\hline
 \end{tabular}}
  \caption{Accuracy of \RetrievalScoring with gt on seen data, unseen data, and full test data.}
  \label{table:Accuracy of NSPlan with gt on seen data and unseen data.}
 \vspace{-3mm}
 \end{table}
 
  \subsection{Analysis of the sequence number $k$ in the reasoner of \RetrievalScoring}
% For our generative model, in addition to measuring each answer directly with a likelihood score, we also conduct experiments using the same reasoner as our \RetrievalScoring baseline to determine the answer based on top-k generative sequences. The results in Table \ref{appendices:table:unseen or seen} show that adding a reasoner can improve the accuracy of all generative models on the test dataset, especially for the \UniVLProphetNet, making it as good as the \RetrievalScoring model. And in the case of only using top-1 sequence, \UniVLProphetNet with reasoner achieves the best results compared to other baselines. We also observe a phenomenon that the generative models with reasoner decrease in accuracy as k increases, while the performance of the \RetrievalScoring model gets better when k increases.

We study the influence of different $k \in \{1, 5, ..., 50\}$ in the second retrieval stage of \RetrievalScoring based on top-50 first-stage retrieval results. In the left of Figure \ref{fig:top-50 results}, we can find that when k is 15, the accuracy of \RetrievalScoring on planning QA test reaches its best as 64.90\%.  In another case that the final sequences are selected from the top-100 retrieved sequences of the first stage, it gets its best accuracy of 61.18\% when k is 55. 
\label{comparison}

%   \begin{table}[h]
%   \vspace{-1mm}
%   \centering

%   \vspace{-1ex}

%   \adjustbox{max width=\columnwidth}{
%   \begin{tabular}{|l|c|c|c|}
% \hline
% \multicolumn{1}{|c|}{\multirow{2}{*}{Method}} & \multirow{2}{*}{\begin{tabular}[c]{@{}c@{}}\AttentionGRU + Reasoner\\ (Top-1, Top-5, Top-10)\end{tabular}} & \multirow{2}{*}{\begin{tabular}[c]{@{}c@{}}\UniVLProphetNet + Reasoner \\ (Top-1, Top-5, Top-10)\end{tabular}} & \multirow{2}{*}{\begin{tabular}[c]{@{}c@{}}\RetrievalScoring\\ (Top-1, Top-5, Top-10)\end{tabular}} \\
% \multicolumn{1}{|c|}{} &  &  &  \\ \hline
% Full Accuracy(\%)  & 51.76, 32.54, 29.21 & 63.72, 60.78, 60.19 & 60.98, 63.33, 63.72 \\ \hline
% Seen Accuracy(\%) & 44.62, 28.10, 23.96 & 62.80, 58.68, 60.33 & 62.80, 65.28, 65.28 \\ \hline
% UnSeen Accuracy(\%) & 53.98, 33.93, 30.84 & 64.01, 61.44, 60.15 & 63.23, 62.72, 60.41 \\ \hline
% \end{tabular}
% }
%   \caption{Accuracy on seen data, unseen data, and full test data.}
%   \label{appendices:table:unseen or seen}
%  \end{table}
 
 \begin{figure}[htbp]
\centering
\begin{minipage}[t]{0.48\linewidth}
\centering
\includegraphics[width=5cm]{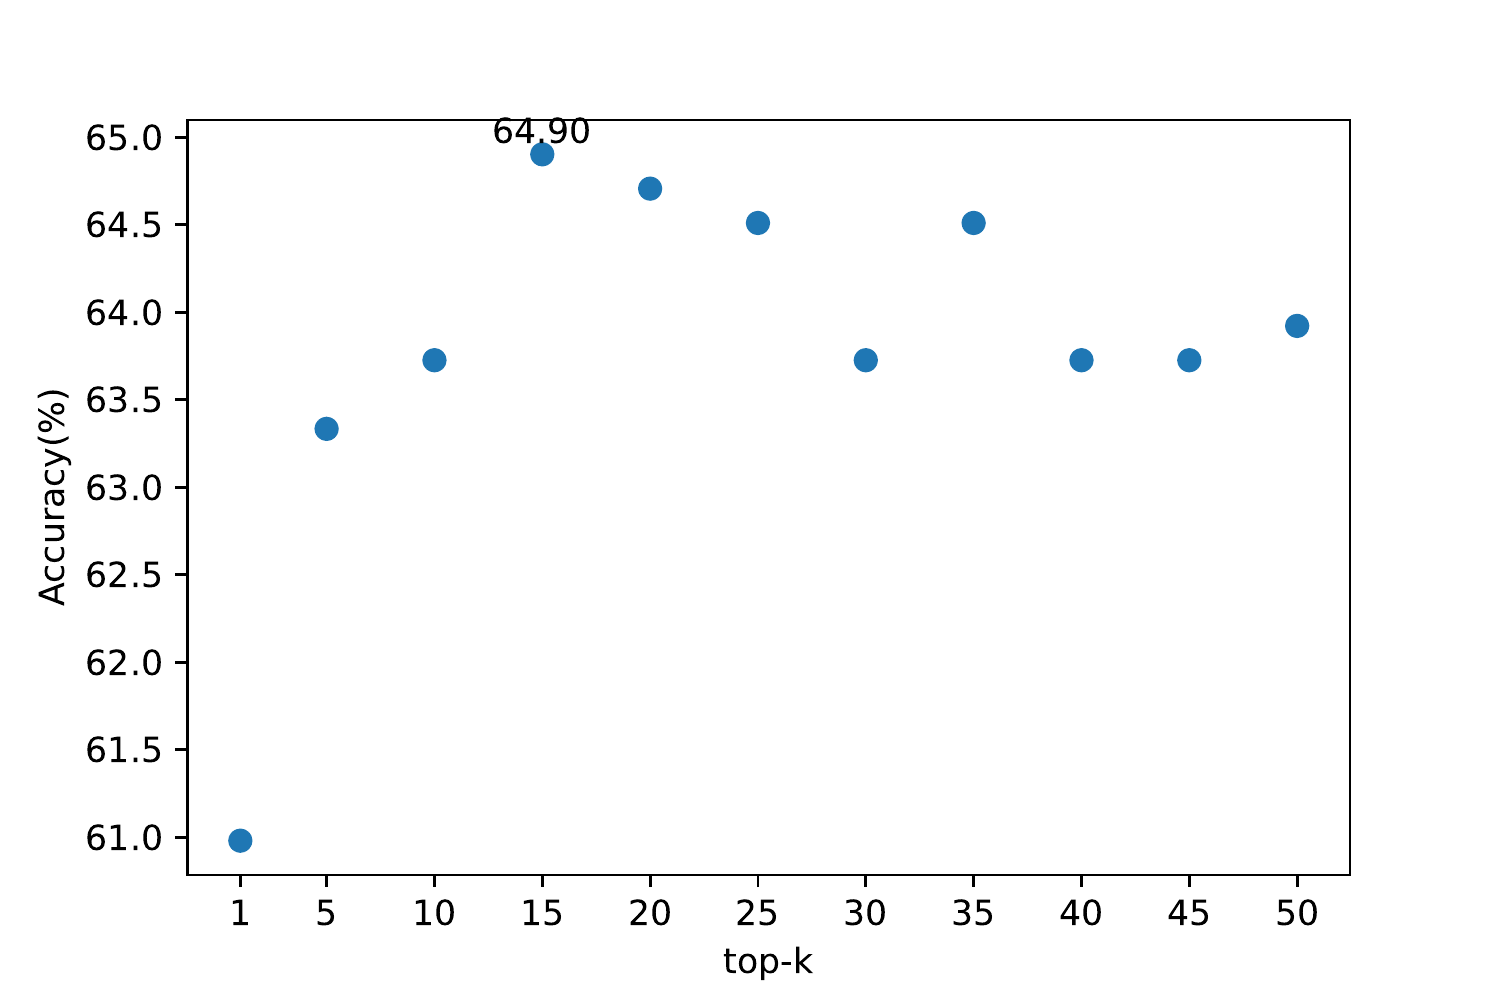}
%\caption{World Map}
\end{minipage}
\begin{minipage}[t]{0.48\linewidth}
\centering
\includegraphics[width=5cm]{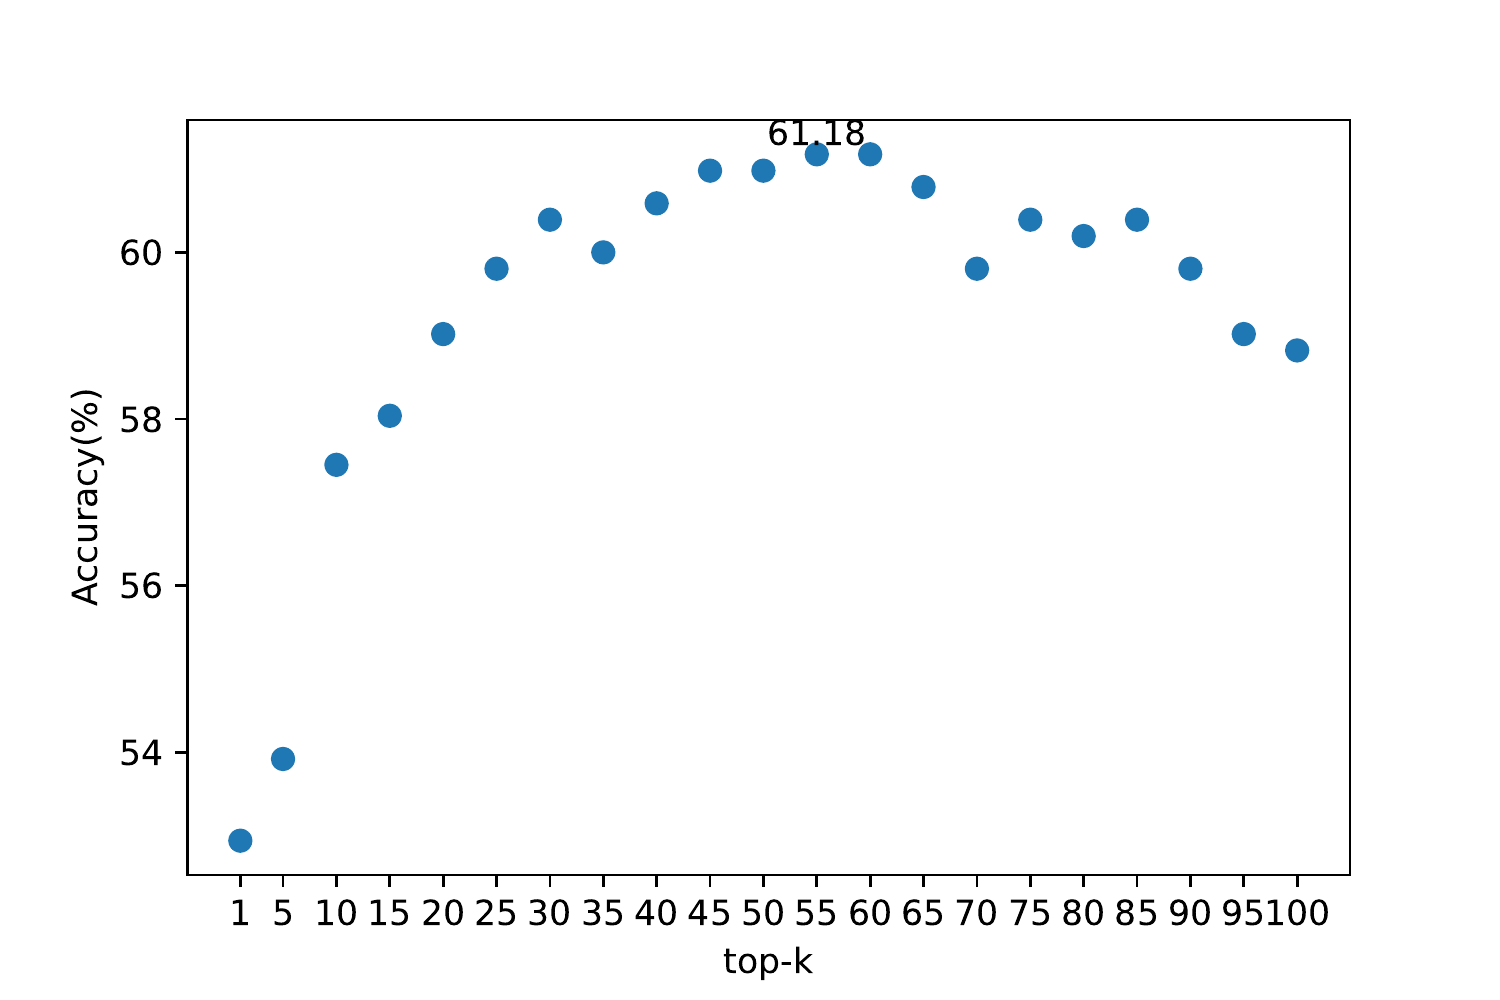}
\end{minipage}
\caption{The influence of selection of k}
\label{fig:top-50 results}
\end{figure}

% \begin{figure}[h]
%    \centering
%    \includegraphics[width=\linewidth]{diagrams/top-50.pdf}
%    \caption{The influence of selection of k.}
%    \label{fig:top-50 results}
%\end{figure}

  % evaluate top-k action seqs
\begin{table*}[!htb]
\vspace{-1ex}
\begin{center}

%\vspace{-1ex}

\resizebox{\textwidth}{!}{
\begin{threeparttable}
\scalebox{1}{\begin{tabular}{|c|l|c|c|c|c|c|c|c|c|}
\hline
\multicolumn{1}{|c|}{\multirow{2}{*}{}} & \multirow{2}{*}{Method} & \multicolumn{6}{c|}{Quality} & \multicolumn{2}{c|}{Diversity} \\ \cline{3-10} 
\multicolumn{1}{|c|}{} &  & precision & \multicolumn{1}{c|}{recall} & \multicolumn{1}{c|}{seq-item-acc} & seq-hits@10 & BLEU1 & BLEU2 & \multicolumn{1}{c|}{Dist1} & Dist2 \\ \hline

\textit{Methods using}  & video-level feature search &22.76&22.40&5.58&8.55&22.43&9.31 &58.70&88.11\\
\textit{low-level visual features only} & frame-level feature alignment &21.99&22.02&4.92&11.11&22.08&9.11&57.88&87.97 \\
\hline
 &\prototype\_\bmTF &29.14&25.03&7.47&18.80&22.69&9.73&19.21&55.09\\
\textit{Methods using} & \slowFast\_\bmTF &29.51&24.52&8.00&19.66&22.21&9.74&23.76&59.08 \\
\textit{action recognition and text retrieval}&\itd\_\bmTF &30.29&25.31&8.11&22.22&22.85&10.02&23.22&57.92 \\ 
&\uniVL\_\bmTF &37.28&30.60&9.60&20.51&28.22&12.18&19.65&54.37 \\ 
&*gt\_\bmTF &77.80&66.87&22.49&69.23&59.64&28.99&20.03&55.59 \\ 
\hline
&\prototype\_\bmTF + OTAM &29.59&25.28&8.01&26.50&22.90&10.19&19.36&54.48\\
\textit{Methods adding}&\prototype\_\bmTF + OTAM\_Rule &29.67&25.41&8.19&27.35&23.08&10.37&20.40&55.31\\
\textit{re-ranking}
&\itd\_\bmTF + OTAM &30.89&25.85&8.95&28.21&23.26&10.76&23.75&57.22\\
&\itd\_\bmTF + OTAM\_Rule &30.88&25.89&9.18&29.91&23.28&10.93&23.70&57.10\\
&\uniVL\_\bmTF + OTAM\_Rule
&37.44&30.82&10.14&26.50&28.50&12.85&18.93&52.35\\
&*gt\_\bmTF + OTAM\_Rule &77.13&66.93&24.37&82.91&59.97&30.45&20.35&54.54\\
\hline
\textit{Methods adding}&\prototype\_\bmTF\_Intention + OTAM\_Rule &39.65&\textbf{39.80}&10.32&33.88&\textbf{38.73}&\textbf{17.36}&32.86&\textbf{69.96}\\
\textit{intent aligning}&\itd\_\bmTF\_Intention + OTAM\_Rule &39.91 &35.48 &11.11 &\textbf{36.36} &33.87 &15.70&\textbf{33.05}&67.41\\
&\uniVL\_\bmTF\_Intention + OTAM\_Rule& 41.16&35.68&\textbf{11.26}&34.71&34.05&15.85&28.02&62.55\\
&*gt\_\bmTF\_Intention + OTAM\_Rule &73.90&64.86&24.00&77.69&59.34&29.83&20.90&56.07\\

\hline
\end{tabular}}
  \begin{tablenotes}    %添加脚注
        \footnotesize              
        \item[1]Method beginning with *gt means that it uses ground truth observed actions as the input of \bmTF search, which can be considered as upper bounds for methods using action recognition.
      \end{tablenotes}         
\end{threeparttable}       
}
\caption{Study of knowledge base retrieval}
\label{table:Results of knowledge base retrieval}
\end{center}
%\vspace{-3ex}
\end{table*}
\FloatBarrier

% \subsection{Additional RQs}
% \subsubsection{Target Action Distribution of Generative Models against the ones in training and the ones in ground truth}
% \begin{figure}[h]
%     \centering
%     \includegraphics[width=\linewidth]{latex/diagrams/action_distribution.PNG}
%     \caption{Action Distribution}
%     \label{fig:action_distribution}
% \end{figure}
% \terry{It is a bit hard to tranform the data to a whole table or chart, as we need to compare the distributions of generative models to the training distribution and the ground truth seperately.}
% Some observation from the action distributions in Figure \ref{fig:action_distribution}: \AttentionGRU failed to learn the planning and results in unreasonable generation. \UniVLProphetNet tends to generate more actions appearing in the training data. However, their frequency distributions over the ground truth are not that significant.

\section{Symbolic Planing}
\label{appendix:symblic_planning}
 \begin{table}[h]
  \vspace{-1mm}
 \centering

 \vspace{-1ex}

 \adjustbox{max width=\columnwidth}{
 \begin{tabular}{|c|c|c|c|}
 \hline
 \row{Method} & \RetrievalScoring & + state aligner & + state aligner-gt \\ \hline
 Accuracy(\%) & 63.72  & 54.10  & 81.96 \\\hline
 \end{tabular}}
  \caption{Effect of symbolic components of action in KB}
  \label{table: Effect of symbolic components of action in KB}
 \vspace{-3mm}
 \end{table}

% \paragraph{\textbf{RQ4: Effect of symbolic components of action in KB. }}
We utilize the symbolic preconditions and operations <PRE, ADD, DEL> of action classes mentioned in Section \ref{sec:mkb}. Specifically, these symbolic operations can be seen as the transfer of states affected by the action. In total, we design 31 template states for the task, which can be found in Appendix \ref{state_template}. We further propose an algorithm to generate the initial and final states of the action sequence using these state transfers. The pseudocode for the state generator can be found in Appendix \ref{appendix:state_generator}. Given an action sequence, we first infer the initial states of the action sequence based on the precondition set and add the effect set of all actions. Then, we reason from the initial states, removing the corresponding deletion effect and adding the add effect for each action, and finally the remaining state as the 
final states when all actions are completed.

\subsection{State Generator}
\label{appendix:state_generator}
We design a state generator algorithm as shown in Algorithm \ref{alg:StateGenerator}.

\begin{algorithm} 
 \SetAlgoNoLine  %去掉之前的竖线
 \caption{StateGenerator}
 \label{alg:StateGenerator}
 
  \KwIn{Action sequence $As = {a_1,a_2,\ldots ,a_n}$, and symbolic components $\left < pre^{a_i}, add^{a_i}, del^{a_i}\right >$ for each action $a_i$,
       where $pre^{a_i}$, $add^{a_i}$, $del^{a_i}$ are sets of states} 
  \KwOut{init states $S_{init}$, final states $S_{final}$} 
    $S_{init}= pre^{a_1}$; \\
    $S_{Add} = add^{a_1}$; \\
    \For{$i=2;i \le n;i++$} 
    { 
        $CurPre = pre^{a_i}$; \\ 
        \For {state $s \in CurPre$} 
        {   
            \If{$s \notin S_{init}$ and $s \notin S_{Add}$} 
            { 
                Append $s$ to $S_{init}$; \\ 
            } 
        } 
        Extend $add^{a_i}$ to $S_{Add}$;\\
    } 
    $S_{cur} = S_{init}$;\\
    \For{$j=1;j \le n;j++$} 
    {
        $CurAdd = add^{a_j}$;\\
        $CurDel = del^{a_j}$;\\
        \For {state $s \in CurDel$}
        {
            \If {$s \in S_{cur}$}
            {
               Remove $s$ from $S_{cur}$;\\
            }      
        }
        Extend $CurAdd$ to $S_{cur}$;\\
    }
    $S_{final} = S_{cur}$;\\
    return $S_{init}, S_{final}$; \\ 
\end{algorithm}

% By adopting this algorithm, we can generate the initial states of all choices about possible future sequences and the final states of the predictive observed action sequence. One way to exploit the action states knowledge is to use a supervised learning paradigm,  which trains a model to learn a mapping from the video input to the final states of the observed action sequence. The final states ground truth label is obtained by using the state generator algorithm, which first infers the initial states of the full ground truth action sequence, then starts from the initial states, infers the final states of observed action sequence corresponding to the input video. We can align these final states of the input video with the generated initial states of the four choices about future action sequences. 
By adopting this algorithm, we can generate the initial states of all choices about possible future sequences and the final states of the observed action sequence. To exploit these states' information, we add a state aligner score into the answer selection module, which measures how well the final states of the input video match the initial states of each choice. One way to get the final states given an input video is to train a model that directly predicts the final state labels. We compare the performance of the method adding \itd-based state generation model and state aligner with our \RetrievalScoring. Besides, we also report the performance of the method using the ground truth final states obtained by inferring from the ground truth observed action sequence. The results in Table \ref{table: Effect of symbolic components of action in KB} show that adding a state aligner hurts the performance, which is mainly due to the low accuracy of \itd-based state generation (e.g. ACC@5 is lower than 0.3). However, we can also observe that if we use the ground truth final states, the state aligner can be quite effective, which shows that the upper bound of leveraging the action states aligner is very high. This is a powerful proof of the effectiveness of action states knowledge. 
% What remains to do for the task is to refine the video final states recognition or the action sequence forecasting model for the better performance.

\subsection{State Template}
\label{state_template}
State Templates =  \{Container(x), *CapacityIncreased(x), CapacityDecreased(x), IsOpen(x), IsCloased(x), IsOn(x), IsOff(x), IsEaten(x), IsAwake(P), IsSleeping(P), Food(x), *Watched(P, x), Talked(P), IsFixed(x), IsBroken(x), Clothes(x), Wearing(P, x), At(x, place), Played(P, x), IsWet(x), InHand(P, x), Reachable(P, x), IsWarmed(P), IsTidy(x), IsMessy(x), IsClean(x), IsDirty(x), IsSitting(P), IsStanding(P),  GetInfoFrom(x, P), Worked(P, x), IsHappy(P)\}, 

where P refers to a person, and x refers to an object. We can also get the specific state by substituting the specific object for x, for example, IsOpen(x) to IsOpen(door)\}.  

There is one example of action's precondition set, delete effect set and add effect set:

\begin{itemize}
    \item \textbf{Action}: Closing a door, 
    \item \textbf{Precondition set}: IsOpen(x)\&Person(P), \item \textbf{Delete effect set}: IsClosed(x)
    \item \textbf{Add effect set}: IsOpen(x)
    \item \textbf{args}: Door
\end{itemize}

\section{Detailed Examples}
\label{more_examples}
We provide examples of Top-10 future action sequences from our baselines in Figures \ref{example_1}, \ref{example_2} and \ref{example_3}. The actions in orange represent future actions, while the actions in BLEU represent the initial observed actions for \RetrievalScoring retrieval. The scoring functions of \UniVLProphetNet and \AttentionGRU are based on log-likelihood, while the score we report in \RetrievalScoring are from $s_{rank}$ in Equation \ref{equation:retrieval_final_score}. We highlight the explainability of \RetrievalScoring by showing its diverse retrieved action sequences and reasonable scores. To validate future action sequences, we use different symbols to represent the correctness against the ground truth: the single red cross means wrong future action sequences; the single green tick means correct future action sequences; the combination of stick and cross means the future action sequence including other actions beside the ground truth or in wrong orders. Although cosine similarity scores between baseline future action sequences and ground truth can be used to evaluate the quality, we consider current representation is more intuitive.

\begin{figure*}[h]
    \includegraphics[width=\linewidth]{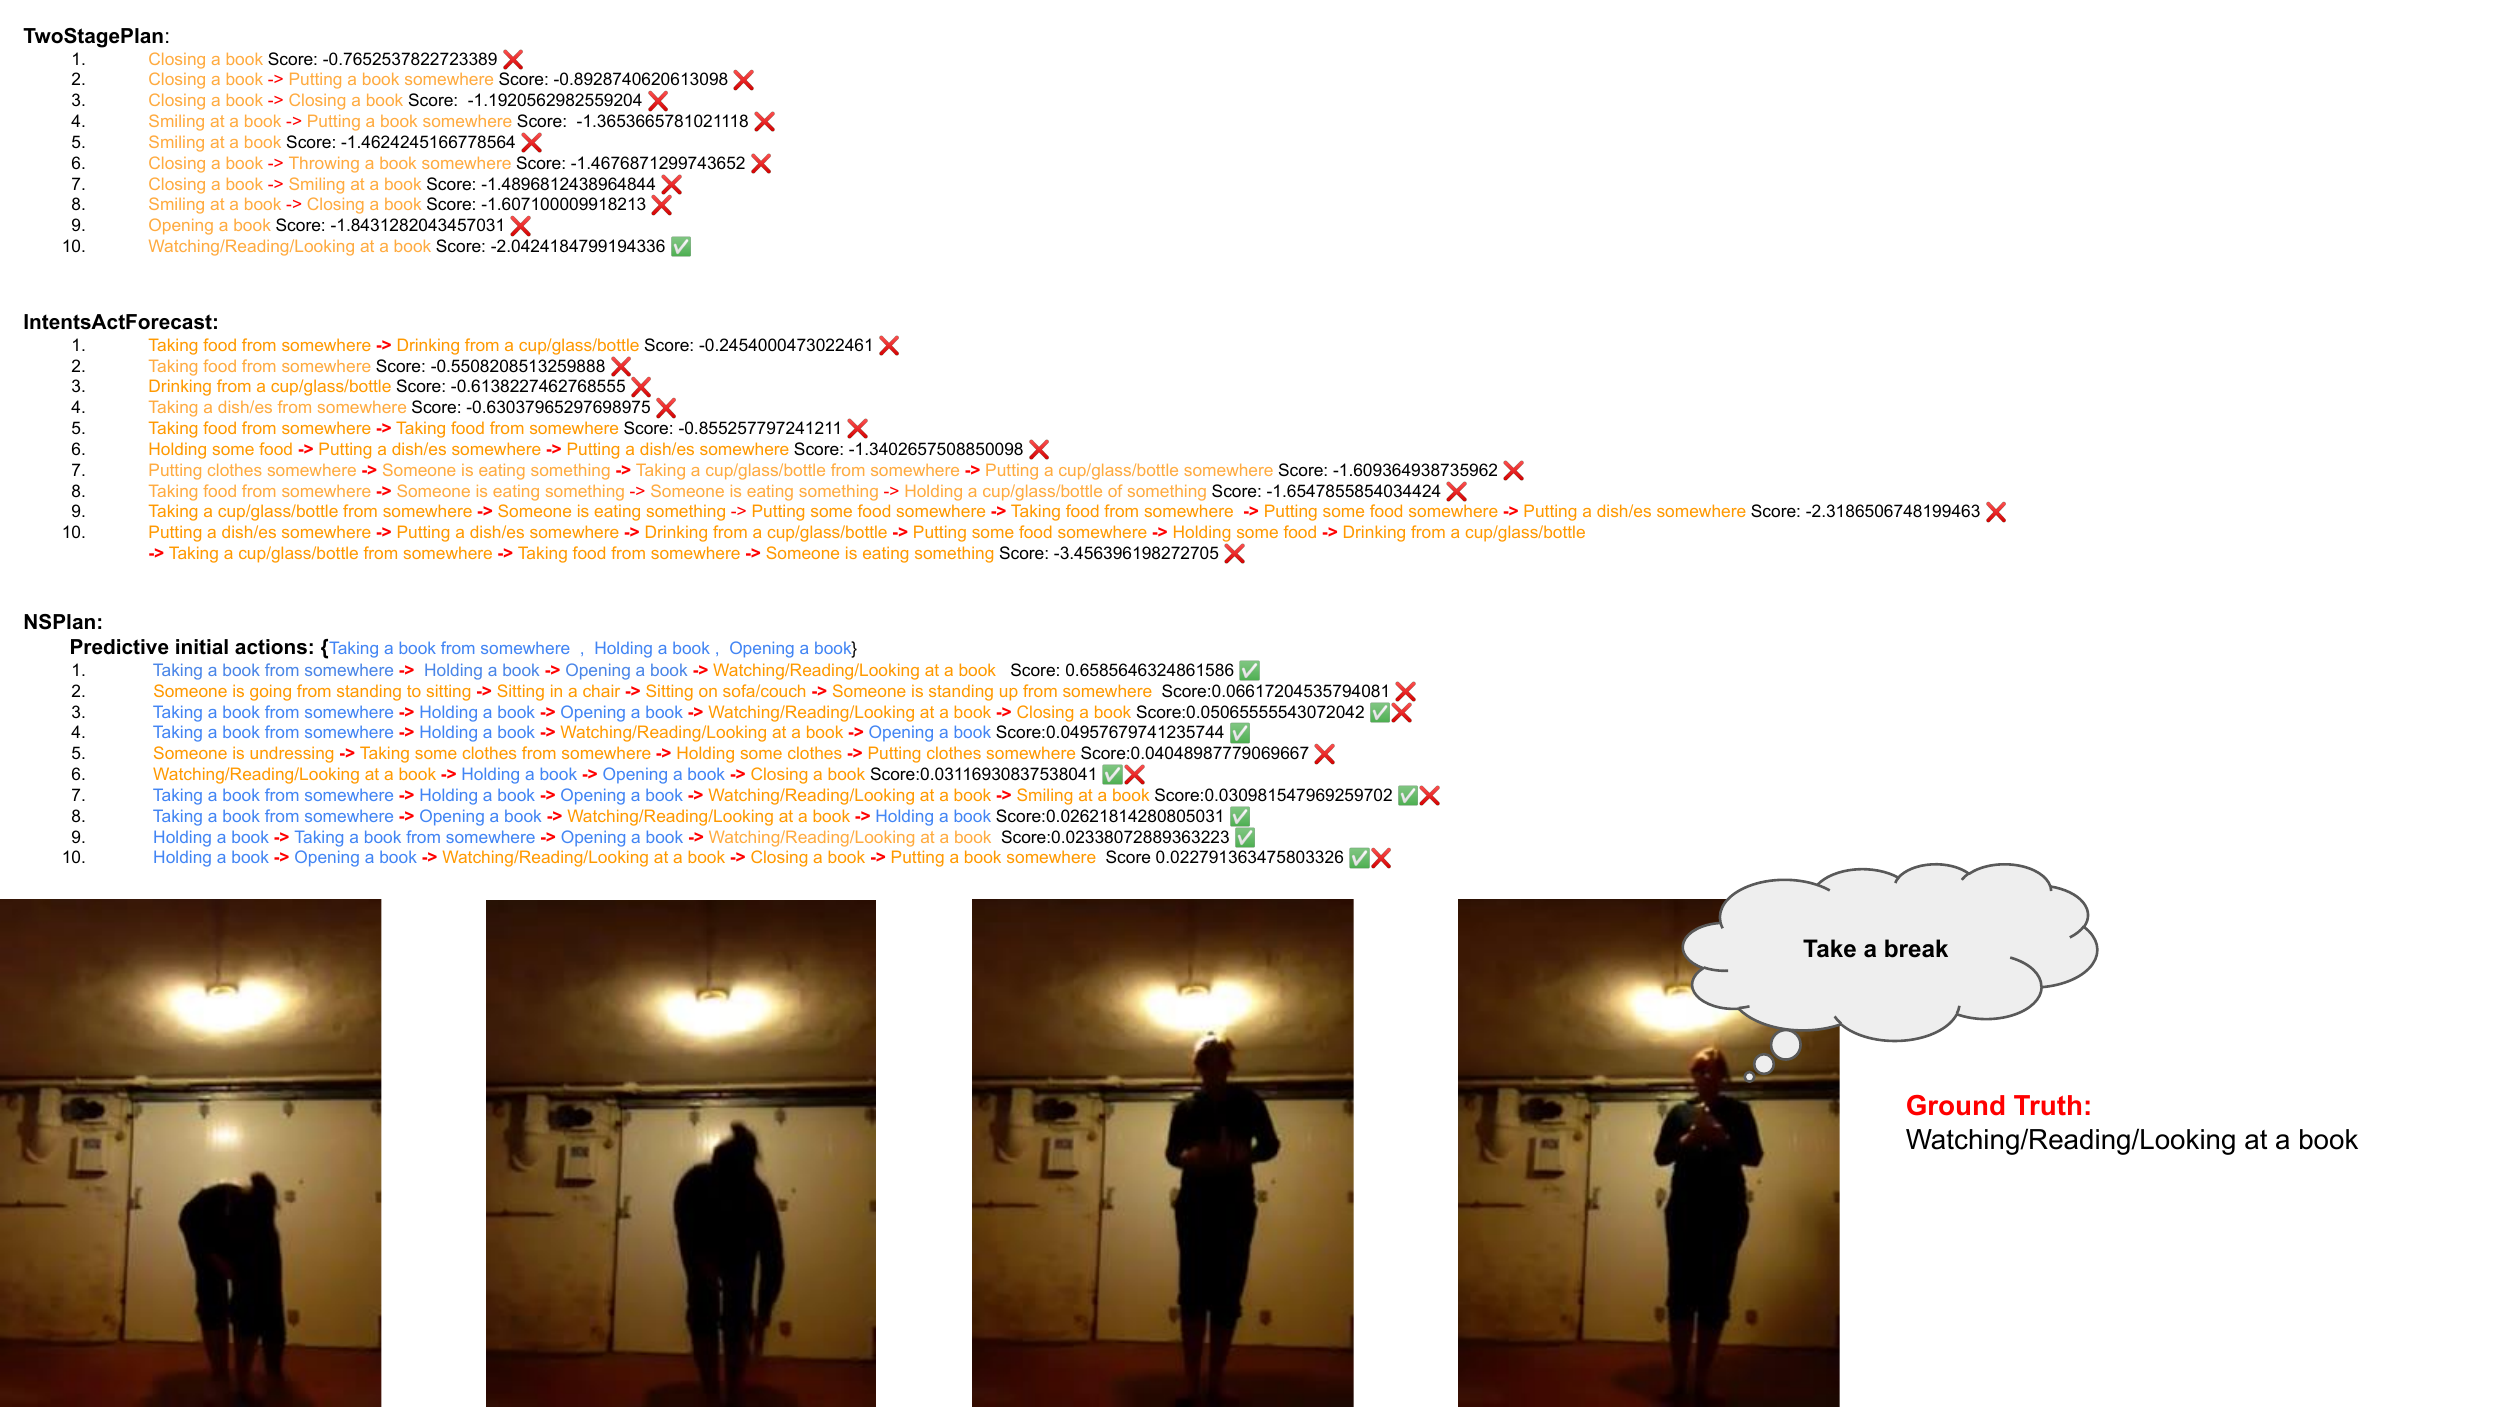}
    \caption{Top-10 Results from different baselines in \charades $G4O9P$ video}
    \label{example_1}
\end{figure*}

\begin{figure*}[h]
    \includegraphics[width=\linewidth]{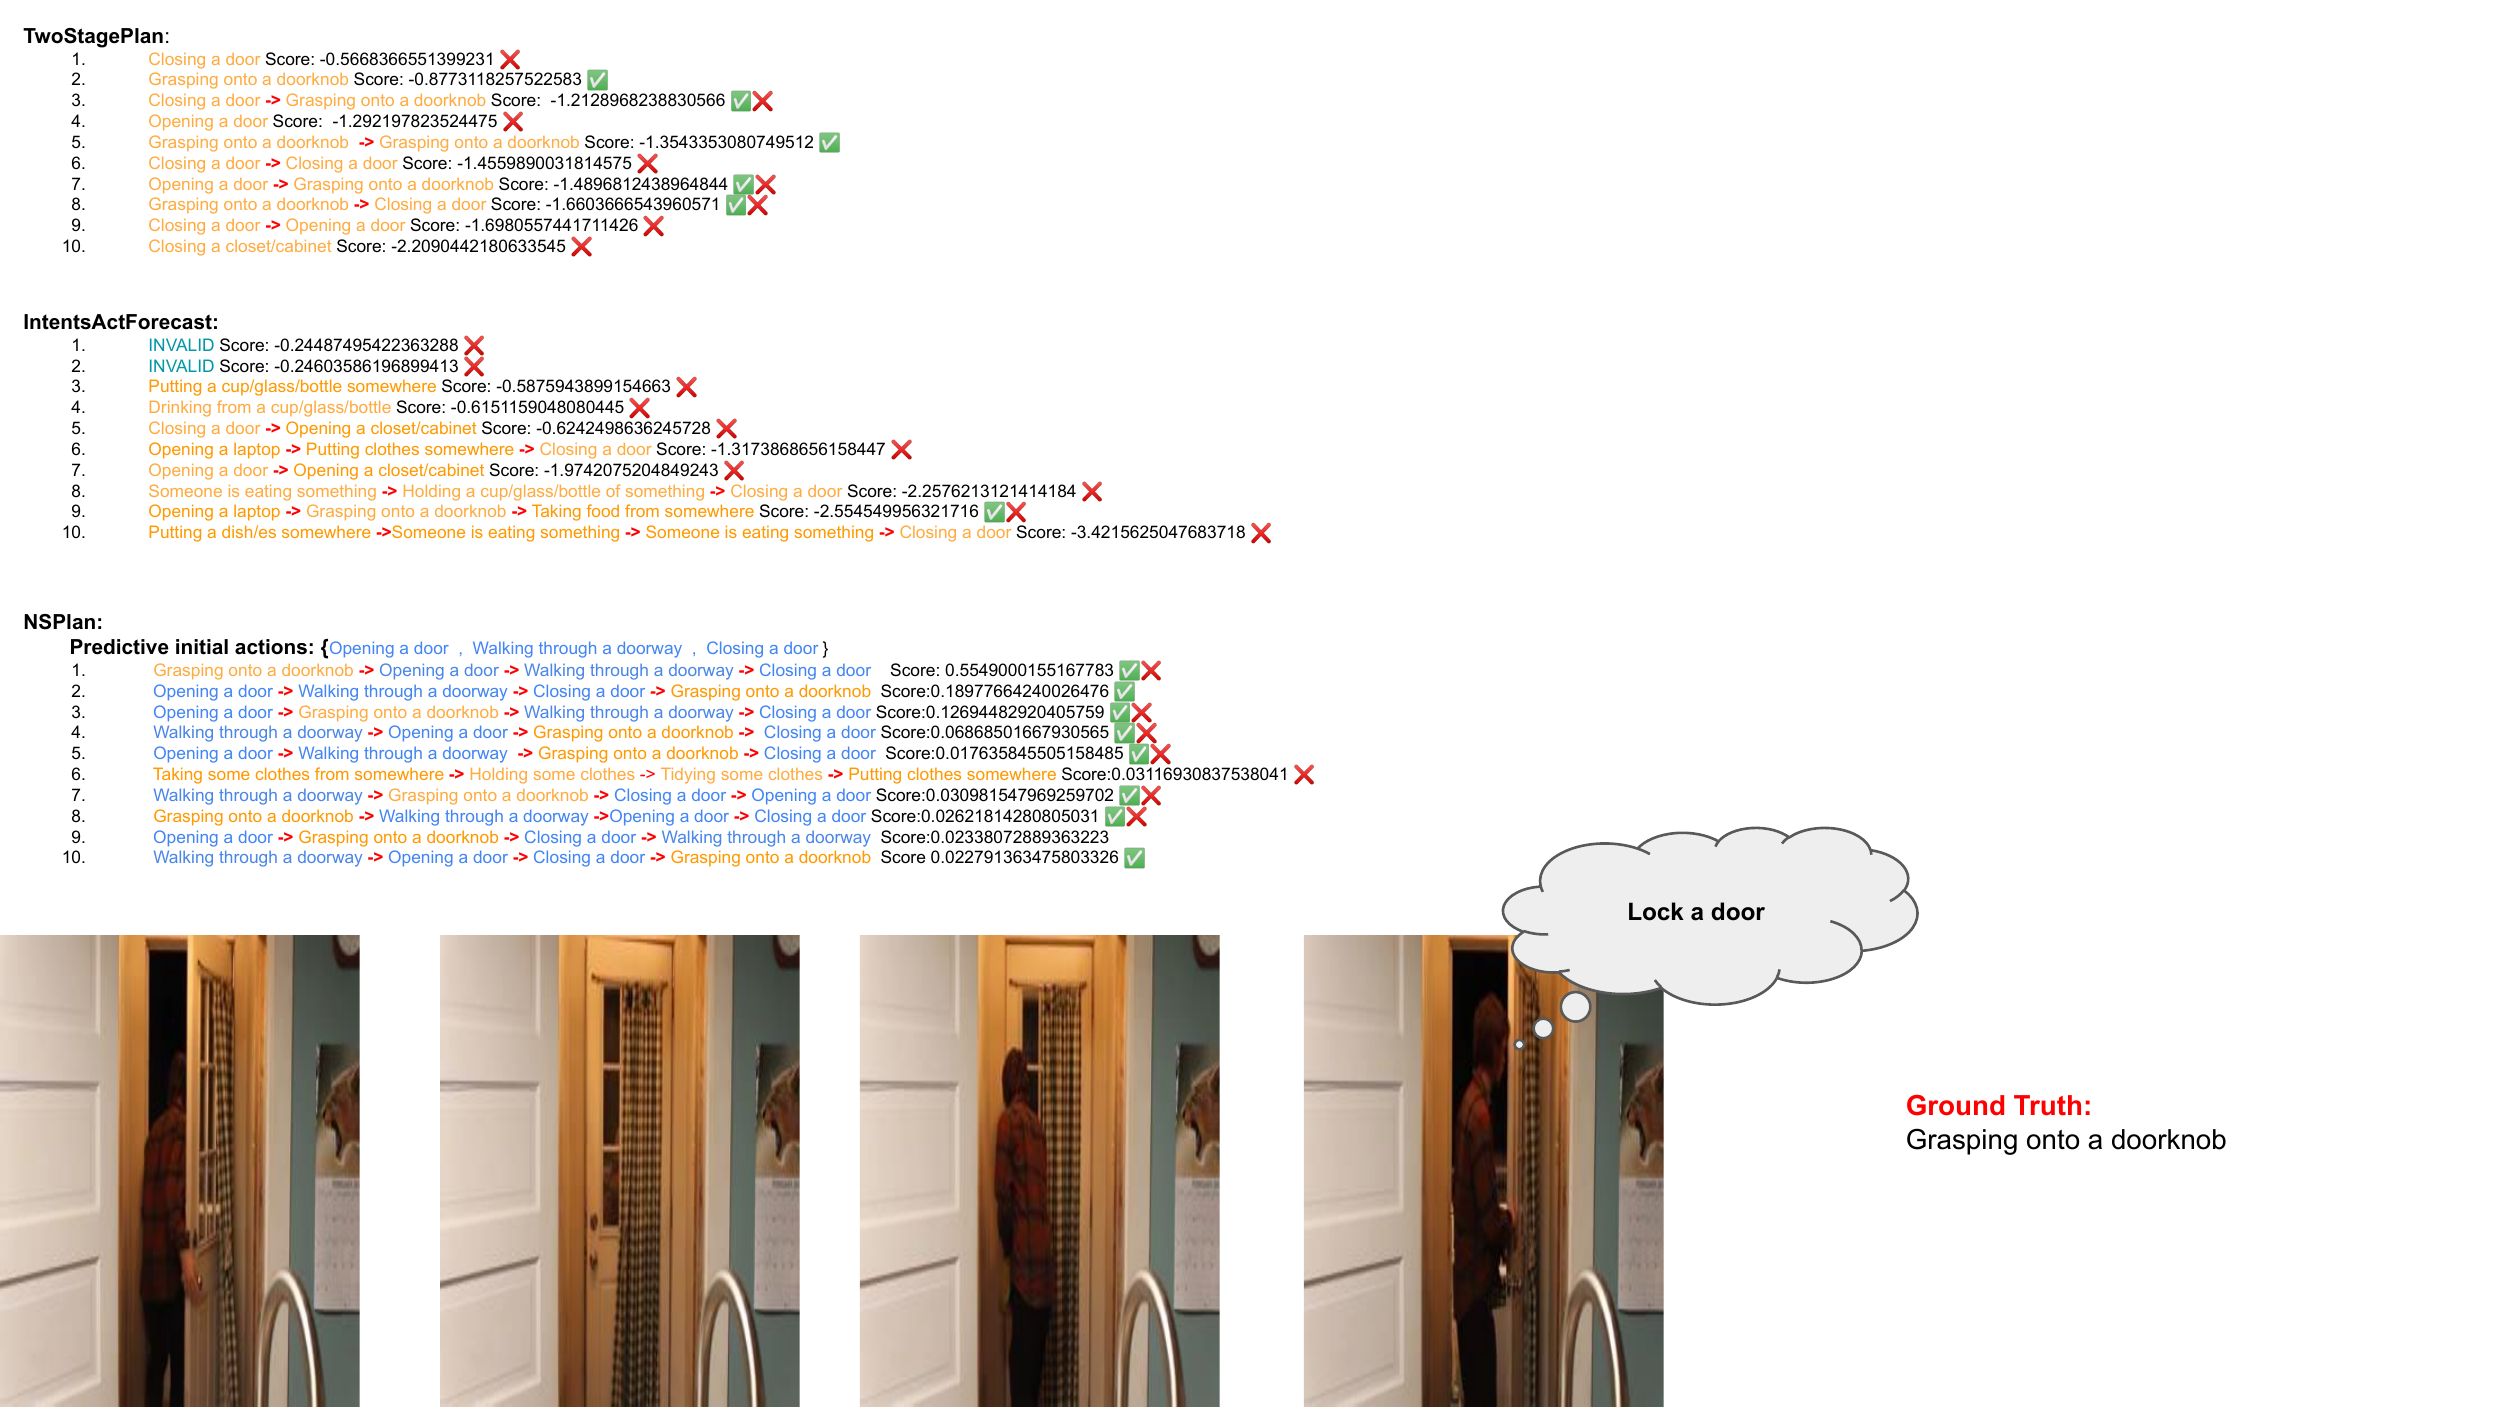}
    \caption{Top-10 Results from different baselines in \charades $2MGC1$ video}
    \label{example_2}
\end{figure*}

\begin{figure*}[h]
    \includegraphics[width=\linewidth]{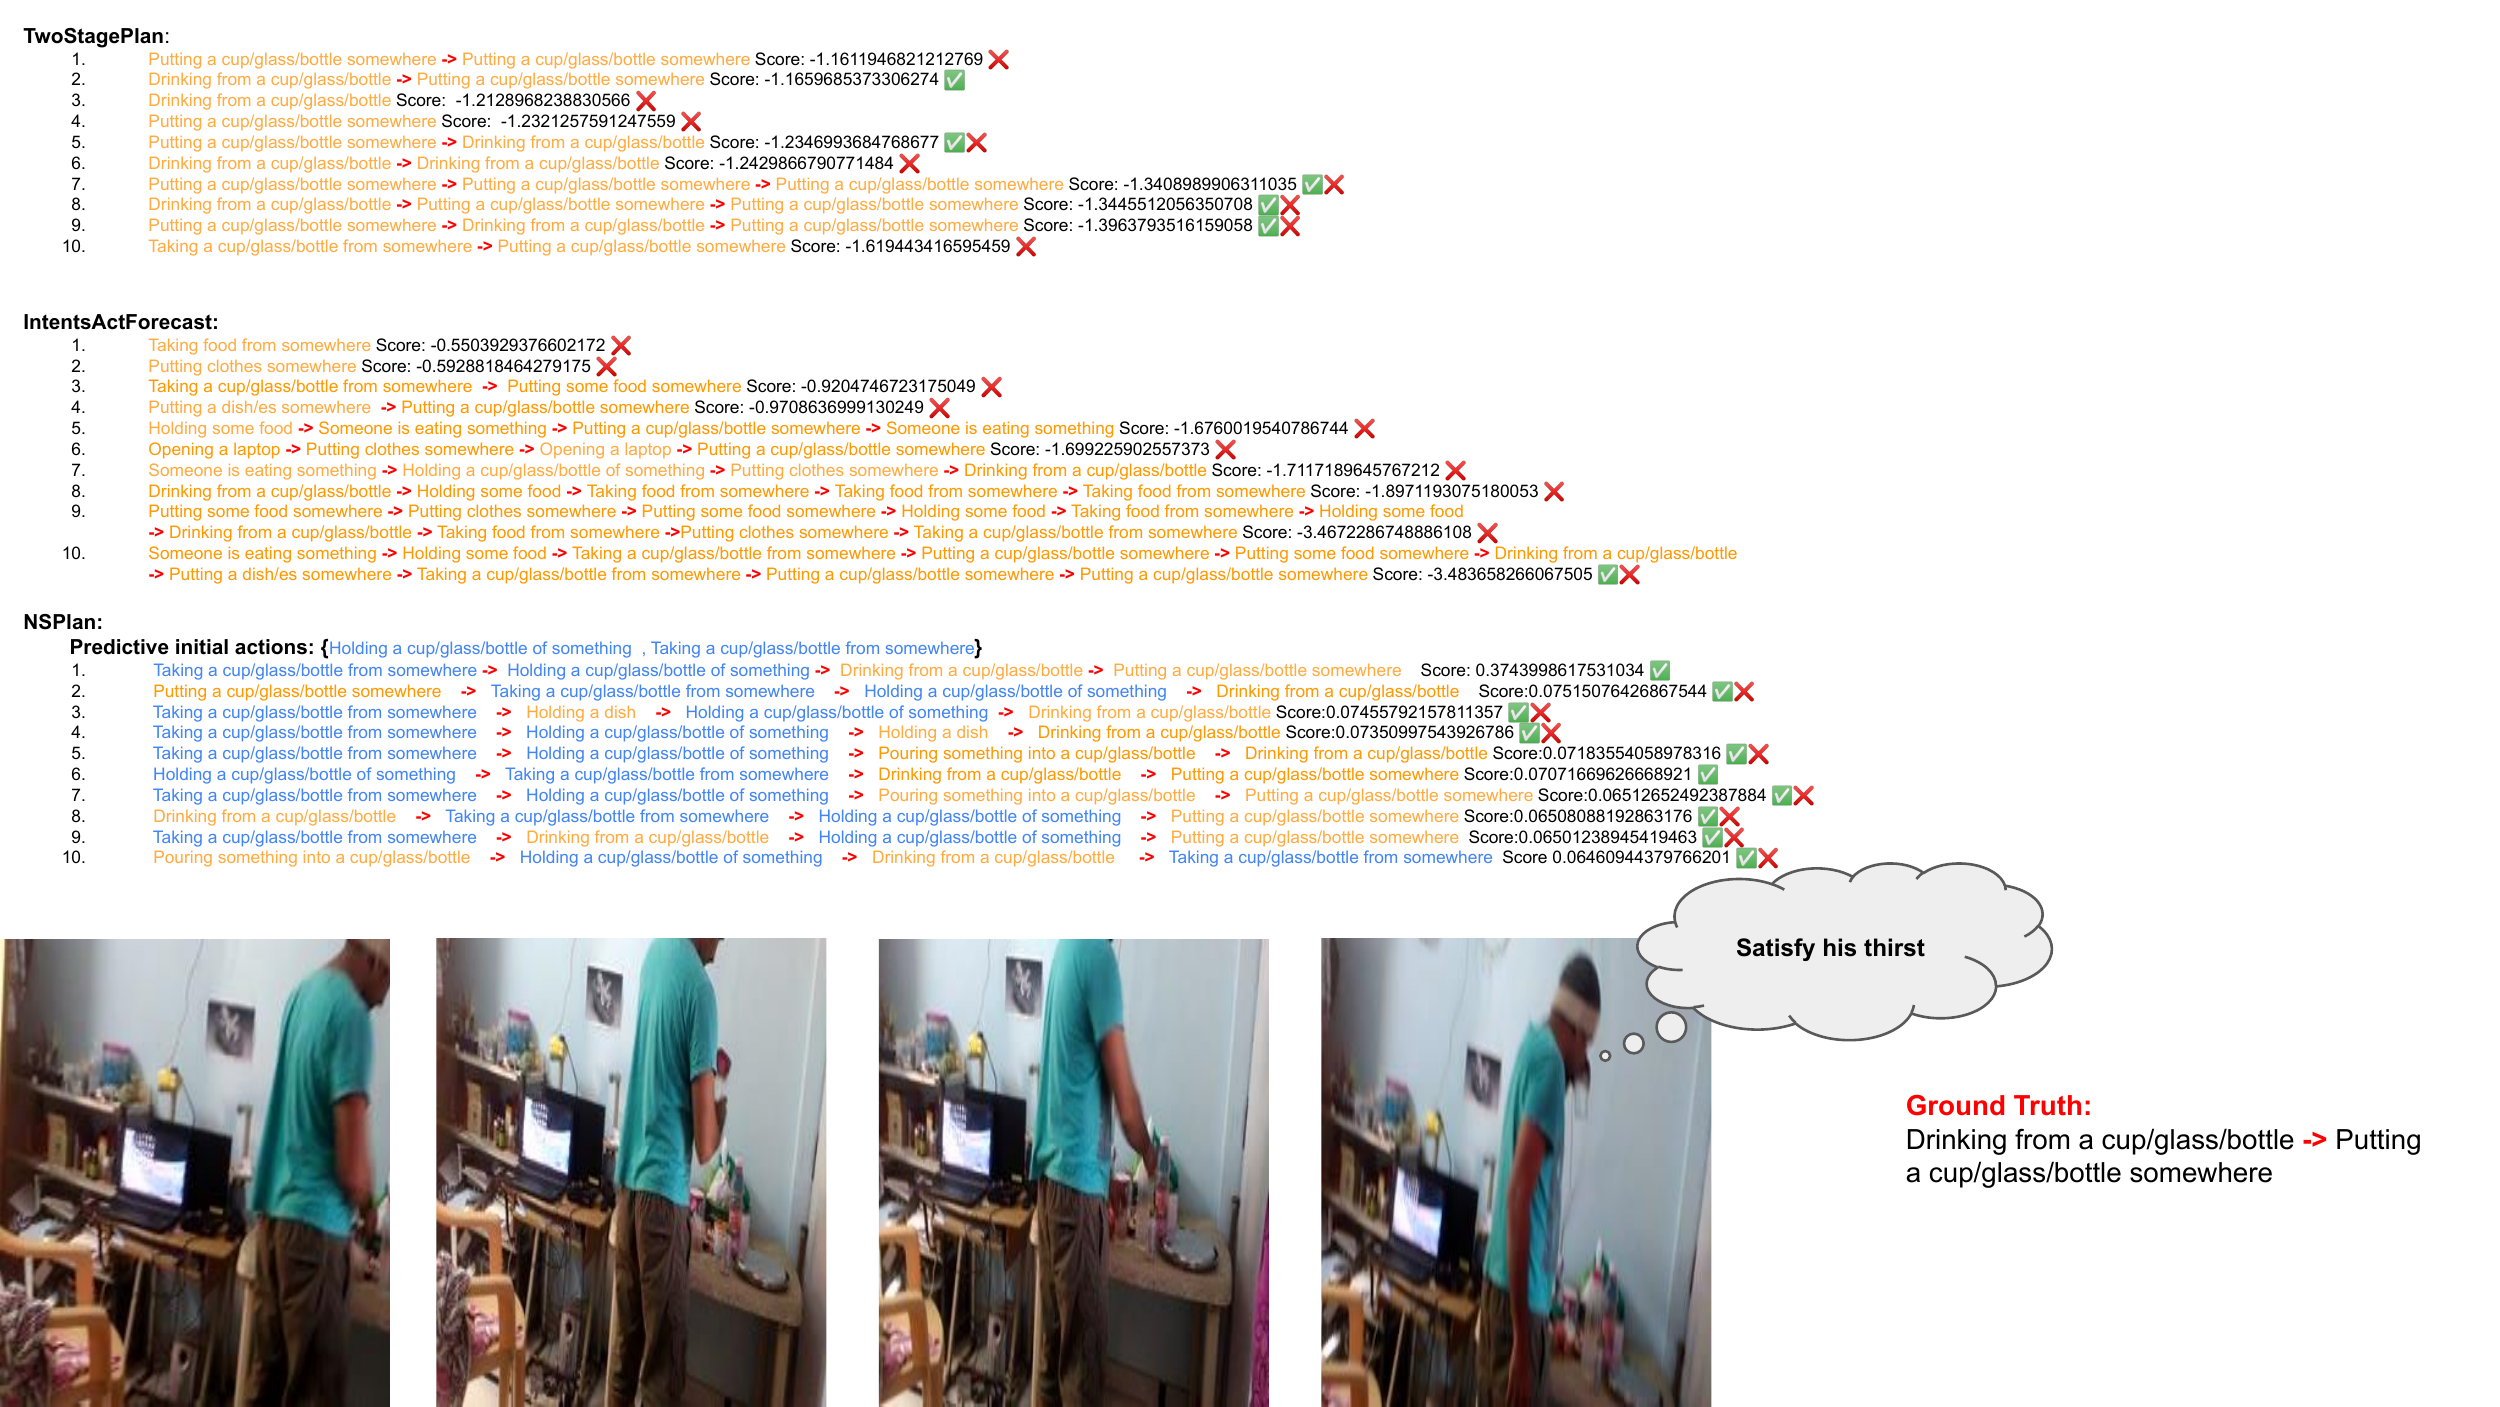}
    \caption{Top-10 Results from different baselines in \charades $S1LQF$ video}
    \label{example_3}
\end{figure*}

% \begin{figure*}[h]
%     \includegraphics[width=\linewidth]{latex/diagrams/example_4.pdf}
%     \caption{1st example of Top-10 Results from different baselines}
%     \label{example_4}
% \end{figure*}

% \begin{figure*}[h]
%     \includegraphics[width=\linewidth]{latex/diagrams/example_5.pdf}
%     \caption{1st example of Top-10 Results from different baselines}
%     \label{example_5}
% \end{figure*}
